# Supplementary material for: The Bring sextic of equilateral pentagons
Source: arXiv:2205.08196 ancillary file (2022-05-17)
Supplement: Supplementary file 1 [file EquilateralPentagonMap.pdf]

# Appendix

Lyle Ramshaw (lyle.ramshaw@gmail.com)

May 14, 2022

This notebook, “EquilateralPentagonMap.nb”, is an appendix in which the calculations of the paper “The Bring sextic of equilateral pentagons” are carried out in detail.

Saving this notebook from within Mathematica — even without having done any evaluations or edits — writes out, as the file “EquilateralPentagonMap.m”, a Mathematica package that exports the conformal mapping projection of the paper as a routine named PoincareCoordinates. That routine is both specified and implemented in section [A9] below. (The package “EquilateralPentagonMap.m” consists of the cells in section [A9] that are InitializationCells, with gray backgrounds.)

Both this notebook and that package assume that the data file “ApproximatingPolynomials.m” will be available in the directory from which the notebook or package is read.

---

## [A1]: The singular points of $E_4$

Figure 3 depicts the polygon space  $E_4$  of equilateral quadrilaterals. It consists of three loops of decomposables, each of which is a geodesic under the bag-of-edges metric  $e_4$ . But what does  $e_4$  say about the three intersection points?

At a singular point of a polygon space, all of the  $n$ -gon’s edges lie along a single line. Perturbing their phases thus leads to a failure-to-close vector that is always orthogonal to that line, to first order. With only one dimension of failure-to-close vectors, rather than two, the dimension of the tangent space jumps up, at a singular point, from  $n - 3$  to  $n - 2$ ; for  $E_4$ , from a tangent line to a tangent plane. And the metric  $e_4$  gives that entire tangent plane a Euclidean structure.

Consider the bottom intersection  $\theta = (0, \pi, 0, \pi)$ , where the four edges of the quadrilateral go back and forth over the same segment twice each way. We can leave  $\theta$  by opening up that quadrilateral into an L that is traveled forward and backward, with the angle of the L at either the left or the right. There are tangent vectors to  $E_4$  at  $\theta$  that point either way — for example,  $\partial_{\text{left}} = (0, 0, 1, 1)$  and  $\partial_{\text{right}} = (0, -1, -1, 0)$ . Their sum  $\partial_{\text{left}} + \partial_{\text{right}} = (0, -1, 0, 1)$  is also a tangent vector to  $E_4$ , lying in the tangent plane to  $E_4$  at the singular point  $\theta$ . Note, though, that we can’t move more than an infinitesimal distance in the direction  $\partial_{\text{left}} + \partial_{\text{right}}$  while remaining in  $E_4$ . Opening up on both sides simultaneously while keeping the edge

lengths fixed produces quadrilaterals that close up only to first order, not to second order. To have them close up, looking like 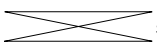, we'd have to lengthen their crossing edges or shorten their noncrossing edges. Such bowtie-shaped quadrilaterals are modeled in the Grassmannian  $\tilde{G}(2, 4)$ , since we can balance the lengthening and shortening so as to preserve the required fixed perimeter.

We can determine the angle between the vectors  $\partial_{\text{left}}$  and  $\partial_{\text{right}}$  by applying, to them and to their sum, our formula in (1) for the bag-of-edges metric  $p_r$ , where  $\mathbf{r} = e(4) = (\frac{1}{4}, \frac{1}{4}, \frac{1}{4}, \frac{1}{4})$ .

Taking the six pairs  $(i, j)$  in (1) in lexicographic order, we have

$p_r(\partial_{\text{left}}) = (0 + 1 + 1 + 1 + 1 + 0)/16 = 1/4$  and  $p_r(\partial_{\text{right}}) = (1 + 1 + 0 + 0 + 1 + 1)/16 = 1/4$ , while  $p_r(\partial_{\text{left}} + \partial_{\text{right}}) = (1 + 0 + 1 + 1 + 4 + 1)/16 = 1/2$ . It follows that  $\|\partial_{\text{left}}\| = \|\partial_{\text{right}}\| = 1/2$ , while  $\|\partial_{\text{left}} + \partial_{\text{right}}\| = 1/\sqrt{2}$ , which implies that  $\partial_{\text{left}}$  and  $\partial_{\text{right}}$  are orthogonal.

Another way to see that this must be so is to reason as follows: For the manifold-with-singularities  $(E_4, e_4)$  to have 48 isomorphisms, we must be able to map the intersection  $\theta$  to any of the three intersections, say  $\theta'$ , and to map the tangent plane at  $\theta$  to the tangent plane at  $\theta'$  in one of eight ways, leaving a binary choice about how to map the two halves of the top loop. In order to have eight different ways to map the tangent plane, all three intersections must be orthogonal.

## [A2]: Figures 2 depicts $E_5^+$

We here verify that Figure 2 depicts the polygon space  $E_5$  with the orientation  $E_5^+$ , the orientation suggested by the argument in Section 7.2. Since Figures 7 and 8 have the same orientation as Figure 2 where they overlap, they also depict  $E_5^+$ .

Let's consider the isosceles trapezoid along the horizontal axis in Figure 2, which has an orange top. If we rotate that trapezoid clockwise (CW) to make its double-length edge horizontal, it has phase vector  $(2\pi/3, \pi, -2\pi/3, 0, 0)$ , taking the edges in rainbow order from red to purple.

- The tangent vector  $(0, 1, 0, 0, 1)$  points along the ditri-pentagon loop that runs diagonally up and to the right. As we move in that direction, we rotate the orange and purple edges CCW in lockstep, passing through a child's house and then leaving the decatract of convex-and-CCW pentagons at the purple-topped isosceles trapezoid.
- The tangent vector  $(0, -1, 0, -1, 0)$  points along the ditri-pentagon loop that runs diagonally up and to the left. As we move in that direction, we rotate the orange and blue edges CW in lockstep, passing through a child's house and leaving the decatract at the blue-topped trapezoid. So the vectors  $(0, 1, 0, 0, 1)$  and  $(0, -1, 0, -1, 0)$ , in that order, are a positive basis for the tangent space to  $E_5$ , when that tangent space has the

orientation of Figure 2.

- The vector  $(1, 1, 1, 1, 1)$  is a positive basis for the real line  $\mathbb{R}$  of rigid rotations.
- The orange edge  $\varepsilon_2$  is CCW from the red edge  $\varepsilon_1$ . Hence, rotating  $\varepsilon_2$  a bit CCW gives a failure-to-close vector that is CCW of the analogous vector that would result from rotating  $\varepsilon_1$  a bit CCW. Thus, the vectors  $(1, 0, 0, 0, 0)$  and  $(0, 1, 0, 0, 0)$ , in that order, are a positive basis for the plane  $\mathbb{C}$  of failures to close.

Figure 2 depicts  $E_5^+$  because this 5-by-5 determinant is positive:

```
In[ ]:= Det[{ {0, 1, 0, 0, 1},
               {0, -1, 0, -1, 0},
               {1, 1, 1, 1, 1},
               {1, 0, 0, 0, 0},
               {0, 1, 0, 0, 0} }]
```

```
Out[ ]:= 1
```

## [A3]: Relations among the vertex angles

We begin with the two equations in (3):

```
In[ ]:= cosSum = 1 + Cos[τ3] + Cos[τ3] Cos[τ4] -
           Sin[τ3] Sin[τ4] + Cos[τ2] + Cos[τ2] Cos[τ1] - Sin[τ2] Sin[τ1]
```

```
Out[ ]:= 1 + Cos[τ2] + Cos[τ1] Cos[τ2] + Cos[τ3] +
           Cos[τ3] Cos[τ4] - Sin[τ1] Sin[τ2] - Sin[τ3] Sin[τ4]
```

```
In[ ]:= sinSum = Sin[τ3] + Sin[τ3] Cos[τ4] +
           Cos[τ3] Sin[τ4] - Sin[τ2] - Sin[τ2] Cos[τ1] - Cos[τ2] Sin[τ1]
```

```
Out[ ]:= -Cos[τ2] Sin[τ1] - Sin[τ2] - Cos[τ1] Sin[τ2] +
           Sin[τ3] + Cos[τ4] Sin[τ3] + Cos[τ3] Sin[τ4]
```

```
In[ ]:= algSubs = Join[Table[Cos[τk] → (1 - tk2) / (1 + tk2), {k, 4}],
                       Table[Sin[τk] → 2 tk / (1 + tk2), {k, 4}]]
```

```
Out[ ]:= {Cos[τ1] → (1 - t12) / (1 + t12), Cos[τ2] → (1 - t22) / (1 + t22), Cos[τ3] → (1 - t32) / (1 + t32), Cos[τ4] → (1 - t42) / (1 + t42),
           Sin[τ1] → 2 t1 / (1 + t12), Sin[τ2] → 2 t2 / (1 + t22), Sin[τ3] → 2 t3 / (1 + t32), Sin[τ4] → 2 t4 / (1 + t42)}
```

```
In[ ]:= commonDenom = Product[1 + tk2, {k, 4}]
```

```
Out[ ]:= (1 + t12) (1 + t22) (1 + t32) (1 + t42)
```

```
In[ ]:= Zcos = commonDenom Factor[cosSum /. algSubs]
```

```
Out[ ]:= 5 + 3 t12 - 4 t1 t2 + t22 + 3 t12 t22 + t32 - t12 t32 - 4 t1 t2 t32 - 3 t22 t32 - t12 t22 t32 -
           4 t3 t4 - 4 t12 t3 t4 - 4 t22 t3 t4 - 4 t12 t22 t3 t4 + 3 t42 + t12 t42 - 4 t1 t2 t42 -
           t22 t42 + t12 t22 t42 + 3 t32 t42 + t12 t32 t42 - 4 t1 t2 t32 t42 - t22 t32 t42 + t12 t22 t32 t42
```

```
In[ ]:= Zsin = commonDenom Factor[sinSum /. algSubs]
Out[ ]:= -2 (t1 + 2 t2 - t1 t2^2 - 2 t3 - 2 t1^2 t3 - 2 t2^2 t3 - 2 t1^2 t2^2 t3 + t1 t3^2 +
2 t2 t3^2 - t1 t2^2 t3^2 - t4 - t1^2 t4 - t2^2 t4 - t1^2 t2^2 t4 + t3^2 t4 + t1^2 t3^2 t4 + t2^2 t3^2 t4 +
t1^2 t2^2 t3^2 t4 + t1 t4^2 + 2 t2 t4^2 - t1 t2^2 t4^2 + t1 t3^2 t4^2 + 2 t2 t3^2 t4^2 - t1 t2^2 t3^2 t4^2)
```

We first use a Gröbner basis to eliminate  $t_4$ . The second argument to GroebnerBasis is a list of variables in which the first is the most expensive, that is, the one that the basis should try the hardest to avoid.

```
In[ ]:= gbOmit4 = GroebnerBasis[{Zcos, Zsin}, {t4, t1, t2, t3}][[1]] // Factor
Out[ ]:= (1 + t1^2)^2 (1 + t2^2)^2 (1 + t3^2)^2 (-15 - 3 t1^2 + 16 t1 t2 + t2^2 -
3 t1^2 t2^2 + 8 t1 t3 + 16 t2 t3 - 8 t1 t2^2 t3 - 3 t3^2 + t1^2 t3^2 - 3 t2^2 t3^2 + t1^2 t2^2 t3^2)
```

The first polynomial in the resulting basis is indeed free of  $t_4$ . We ignore the quadratic factors, which are positive:

```
In[ ]:= relate123 = -Last[gbOmit4]
Out[ ]:= 15 + 3 t1^2 - 16 t1 t2 - t2^2 + 3 t1^2 t2^2 - 8 t1 t3 - 16 t2 t3 + 8 t1 t2^2 t3 + 3 t3^2 - t1^2 t3^2 + 3 t2^2 t3^2 - t1^2 t2^2 t3^2
```

Eliminating  $t_2$  is similar and has a slightly simpler result:

```
In[ ]:= gbOmit2 = GroebnerBasis[{Zcos, Zsin}, {t2, t1, t3, t4}][[1]] // Factor
Out[ ]:= (1 + t1^2) (1 + t3^2)^2 (1 + t4^2)^2
(5 + 9 t1^2 - 3 t3^2 + t1^2 t3^2 - 8 t3 t4 - 8 t1^2 t3 t4 - 3 t4^2 + t1^2 t4^2 - 3 t3^2 t4^2 + t1^2 t3^2 t4^2)

In[ ]:= relate134 = Last[gbOmit2]
Out[ ]:= 5 + 9 t1^2 - 3 t3^2 + t1^2 t3^2 - 8 t3 t4 - 8 t1^2 t3 t4 - 3 t4^2 + t1^2 t4^2 - 3 t3^2 t4^2 + t1^2 t3^2 t4^2
```

## [A4]: Compatible values for $t_2$ and $t_3$

We introduce the new names  $x$  and  $y$  for  $t_1$  and  $t_4$ . We then compute the two possible values for  $t_3$  in terms of  $x$  and  $y$ .

```
In[ ]:= useXY = {t1 -> x, t4 -> y}
Out[ ]:= {t1 -> x, t4 -> y}

In[ ]:= t3vals = Solve[relate134 == 0, t3] /. useXY // Simplify
Out[ ]:= {{t3 -> (4 (1 + x^2) y - Sqrt[15 + 22 y^2 - 9 y^4 - x^4 (-3 + y^2)^2 + x^2 (22 + 60 y^2 + 6 y^4)]) /
((-3 + x^2) (1 + y^2))},
{t3 -> (4 (1 + x^2) y + Sqrt[15 + 22 y^2 - 9 y^4 - x^4 (-3 + y^2)^2 + x^2 (22 + 60 y^2 + 6 y^4)]) /
((-3 + x^2) (1 + y^2))}}
```

The radicand here is the discriminant of relate134 as a quadratic polynomial in  $t_3$ , except that Simplify has pulled out a factor of  $\text{Sqrt}[4] == 2$ :

```
In[ ]:= radQ = Discriminant[relate134, t3] / 4 /. useXY
Out[ ]:= 15 + 22 x^2 - 9 x^4 + 22 y^2 + 60 x^2 y^2 + 6 x^4 y^2 - 9 y^4 + 6 x^2 y^4 - x^4 y^4
```

The possible values for  $t_2$  are symmetric:

```
In[ ]:= t2vals = t3vals /. {t3 -> t2, x -> y, y -> x}
Out[ ]:= {{t2 -> (4 x (1 + y^2) - Sqrt[(15 + 22 x^2 - 9 x^4 + (22 + 60 x^2 + 6 x^4) y^2 - (-3 + x^2)^2 y^4]) /
  ((1 + x^2) (-3 + y^2)))},
  {t2 -> (4 x (1 + y^2) + Sqrt[(15 + 22 x^2 - 9 x^4 + (22 + 60 x^2 + 6 x^4) y^2 - (-3 + x^2)^2 y^4]) /
  ((1 + x^2) (-3 + y^2)))}}
```

To see which signs for the radicals in  $t_2$  and  $t_3$  are compatible, we substitute our two solutions for each into both  $Z_{\cos}$  and  $Z_{\sin}$ . It turns out that  $Z_{\cos}$  doesn't care about the signs, but  $Z_{\sin}$  insists that the signs in the formulas for  $t_2$  and  $t_3$  be the same:

```
In[ ]:= MatrixForm[Table[
  SameQ[0, Simplify[Zcos /. useXY /. t2vals[[i]] /. t3vals[[j]]], {i, 2}, {j, 2}]]
Out[ ]//MatrixForm=
  ( True  True )
  ( True  True )

In[ ]:= MatrixForm[Table[
  SameQ[0, Simplify[Zsin /. useXY /. t2vals[[i]] /. t3vals[[j]]], {i, 2}, {j, 2}]]
Out[ ]//MatrixForm=
  ( True  False )
  ( False True )
```

## [A5]: The first fundamental form of $(E_5, e_5)$

We denote the “**bag-of-edges first fundamental form**” as “bfff”.

```
In[ ]:= halfAngleSubs = {x -> Tan[ξ/2], y -> Tan[η/2]};
In[ ]:= halfAngleBackSubs =
  {Tan[ξ/2] -> x, Tan[η/2] -> y, Cot[ξ/2] -> 1/x, Cot[η/2] -> 1/y};
```

We can set the five phases using either compatible pair of solutions for  $t_2$  and  $t_3$ :

```
In[ ]:= θ[3] = 0;
In[ ]:= θ[4] = 2 ArcTan[t3] /. t3vals[[1]] /. halfAngleSubs;
In[ ]:= θ[5] = θ[4] + η;
In[ ]:= θ[2] = -2 ArcTan[t2] /. t2vals[[1]] /. halfAngleSubs;
In[ ]:= θ[1] = θ[2] - ξ;
```

We compute “bfff” by plugging those phases into the definition of the bag-of-edges metric in (1). That computation itself is straightforward; but we don't print the result, since it is lengthy and opaque.

```
In[ ]:= bfffRaw = Sum[(Dt[θ[j]] - Dt[θ[i]])^2/25, {i, 1, 5}, {j, i + 1, 5}];
```

How can we simplify that result enough to be useful? Invoking `Simplify` or `FullSimplify` in the obvious way doesn't help, since they keep executing indefinitely — apparently exploring countless ways to exploit trigonometric identities. Fortunately, `FullSimplify` does well if we outlaw trigonometry by specifying `Trig → False`.

One tricky point, though: Differentiation has introduced factors of  $\text{Sec}[\xi/2]^2$  and  $\text{Sec}[\eta/2]^2$  into `bfffRaw`. We would prefer to stick entirely with tangents, and we can't leave that chore to `FullSimplify`, since we are forbidding it to use trigonometry. So we apply our own substitution rule that replaces  $\text{Sec}[z]^2$  with  $\text{Tan}[z]^2 + 1$ .

```
In[ ]:= secToTan = Sec[arg_]^(n_ /; EvenQ[n]) → (Tan[arg]^2 + 1)^(n/2);
```

The following line then takes perhaps 15 seconds to do the crucial simplification:

```
In[ ]:= bfff = FullSimplify[bfffRaw /. secToTan, Trig → False]
```

```
Out[ ]:= (Dt[ξ]^2
```

$$\begin{aligned} & \left( 5 \left( -3 + \text{Tan}\left[\frac{\eta}{2}\right]^2 \right) \left( 5 + 9 \text{Tan}\left[\frac{\eta}{2}\right]^2 \right) - \left( 5 + 9 \text{Tan}\left[\frac{\eta}{2}\right]^2 \right) \left( 45 + 17 \text{Tan}\left[\frac{\eta}{2}\right]^2 \right) \text{Tan}\left[\frac{\xi}{2}\right]^2 - \right. \\ & \left. \left( -3 + \text{Tan}\left[\frac{\eta}{2}\right]^2 \right) \left( 5 + 9 \text{Tan}\left[\frac{\eta}{2}\right]^2 \right) \text{Tan}\left[\frac{\xi}{2}\right]^4 - 3 \left( -3 + \text{Tan}\left[\frac{\eta}{2}\right]^2 \right)^2 \text{Tan}\left[\frac{\xi}{2}\right]^6 \right) + \\ & 4 \text{Dt}[\eta] \text{Dt}[\xi] \text{Tan}\left[\frac{\eta}{2}\right] \text{Tan}\left[\frac{\xi}{2}\right] \left( 55 + 50 \text{Tan}\left[\frac{\xi}{2}\right]^2 + 27 \text{Tan}\left[\frac{\xi}{2}\right]^4 - \text{Tan}\left[\frac{\eta}{2}\right]^4 \right. \\ & \left. \left( -3 + \text{Tan}\left[\frac{\xi}{2}\right]^2 \right) \left( 9 + \text{Tan}\left[\frac{\xi}{2}\right]^2 \right) - 2 \text{Tan}\left[\frac{\eta}{2}\right]^2 \left( 5 + \text{Tan}\left[\frac{\xi}{2}\right]^2 \right) \left( -5 + 3 \text{Tan}\left[\frac{\xi}{2}\right]^2 \right) \right) + \\ & \text{Dt}[\eta]^2 \left( -3 \text{Tan}\left[\frac{\eta}{2}\right]^6 \left( -3 + \text{Tan}\left[\frac{\xi}{2}\right]^2 \right)^2 + 5 \left( -3 + \text{Tan}\left[\frac{\xi}{2}\right]^2 \right) \left( 5 + 9 \text{Tan}\left[\frac{\xi}{2}\right]^2 \right) - \text{Tan}\left[\frac{\eta}{2}\right]^2 \right. \\ & \left. \left( 5 + 9 \text{Tan}\left[\frac{\xi}{2}\right]^2 \right) \left( 45 + 17 \text{Tan}\left[\frac{\xi}{2}\right]^2 \right) + \text{Tan}\left[\frac{\eta}{2}\right]^4 \left( 15 + 22 \text{Tan}\left[\frac{\xi}{2}\right]^2 - 9 \text{Tan}\left[\frac{\xi}{2}\right]^4 \right) \right) \right) / \\ & \left( 50 \left( \text{Tan}\left[\frac{\eta}{2}\right]^4 \left( -3 + \text{Tan}\left[\frac{\xi}{2}\right]^2 \right)^2 + \left( -3 + \text{Tan}\left[\frac{\xi}{2}\right]^2 \right) \left( 5 + 9 \text{Tan}\left[\frac{\xi}{2}\right]^2 \right) - \right. \right. \\ & \left. \left. 2 \text{Tan}\left[\frac{\eta}{2}\right]^2 \left( 11 + 30 \text{Tan}\left[\frac{\xi}{2}\right]^2 + 3 \text{Tan}\left[\frac{\xi}{2}\right]^4 \right) \right) \right) \end{aligned}$$

We partition the first fundamental form into its three pieces  $E$ ,  $F$ , and  $G$ .

```
In[ ]:= bE = Coefficient[bfff, Dt[ξ]^2];
```

```
In[ ]:= bF = Coefficient[bfff, Dt[ξ] Dt[η]] / 2;
```

```
In[ ]:= bG = Coefficient[bfff, Dt[η]^2];
```

To quote those formulas in the paper as (8), we use `halfAngleBackSubs` to substitute in the Weierstrass variables  $x$  and  $y$ . To make the symmetries more apparent, we also call `Factor` to expand out the Horner-like nested structure that `FullSimplify` comes up with for polynomials.

`In[ ]:= bE /. halfAngleBackSubs // Factor`

$$\text{Out[ ]} = - \left( \left( 75 + 225 x^2 - 15 x^4 + 27 x^6 + 110 y^2 + 490 x^2 y^2 - 22 x^4 y^2 - 18 x^6 y^2 - 45 y^4 + 153 x^2 y^4 + 9 x^4 y^4 + 3 x^6 y^4 \right) / \left( 50 \left( -15 - 22 x^2 + 9 x^4 - 22 y^2 - 60 x^2 y^2 - 6 x^4 y^2 + 9 y^4 - 6 x^2 y^4 + x^4 y^4 \right) \right) \right)$$

`In[ ]:= bF /. halfAngleBackSubs // Factor`

$$\text{Out[ ]} = - \left( \left( x y \left( -55 - 50 x^2 - 27 x^4 - 50 y^2 + 20 x^2 y^2 + 6 x^4 y^2 - 27 y^4 + 6 x^2 y^4 + x^4 y^4 \right) \right) / \left( 25 \left( -15 - 22 x^2 + 9 x^4 - 22 y^2 - 60 x^2 y^2 - 6 x^4 y^2 + 9 y^4 - 6 x^2 y^4 + x^4 y^4 \right) \right) \right)$$

`In[ ]:= bG /. halfAngleBackSubs // Factor`

$$\text{Out[ ]} = - \left( \left( 75 + 110 x^2 - 45 x^4 + 225 y^2 + 490 x^2 y^2 + 153 x^4 y^2 - 15 y^4 - 22 x^2 y^4 + 9 x^4 y^4 + 27 y^6 - 18 x^2 y^6 + 3 x^4 y^6 \right) / \left( 50 \left( -15 - 22 x^2 + 9 x^4 - 22 y^2 - 60 x^2 y^2 - 6 x^4 y^2 + 9 y^4 - 6 x^2 y^4 + x^4 y^4 \right) \right) \right)$$

Now that `FullSimplify` with `Trig → False` has done the bulk of the simplifying work, we can `FullSimplify` again with the default `Trig → True`. The formulas shrink a bit, but the further reduction is not dramatic:

`In[ ]:= bEfullSimp = FullSimplify[bE]`

$$\text{Out[ ]} = - \left( \left( -24 \left( 1 + 2 \cos[\eta] \right) \cos[\xi] - \frac{6 \left( 1 + 2 \cos[\eta] \right)^2}{1 + \cos[\xi]} + 24 \cos[2\xi] - 32 \sin[\eta]^2 \right) / \left( 50 \left( 3 - 2 \cos[2\eta] + 4 \cos[\xi] + \cos[\eta] \left( 4 + 8 \cos[\xi] \right) - 2 \cos[2\xi] \right) \right) \right)$$

`In[ ]:= bFfullSimp = FullSimplify[bF]`

$$\text{Out[ ]} = - \left( \left( \left( 19 + 14 \cos[\eta] + 4 \cos[2\eta] + 14 \cos[\xi] + 4 \cos[2\xi] \right) \tan\left[\frac{\eta}{2}\right] \tan\left[\frac{\xi}{2}\right] \right) / \left( 25 \left( 3 - 2 \cos[2\eta] + 4 \cos[\xi] + \cos[\eta] \left( 4 + 8 \cos[\xi] \right) - 2 \cos[2\xi] \right) \right) \right)$$

`In[ ]:= bGfullSimp = FullSimplify[bG]`

$$\text{Out[ ]} = - \left( \left( \left( -23 - 14 \cos[\eta] + 6 \cos[2\eta] + 6 \cos[3\eta] - 12 \left( 2 + 2 \cos[\eta] + \cos[2\eta] \right) \cos[\xi] + 2 \left( 1 + 4 \cos[\eta] \right) \cos[2\xi] \right) \sec\left[\frac{\eta}{2}\right]^2 \right) / \left( 50 \left( 3 - 2 \cos[2\eta] + 4 \cos[\xi] + \cos[\eta] \left( 4 + 8 \cos[\xi] \right) - 2 \cos[2\xi] \right) \right) \right)$$

In addition, the formulas then lose some of their symmetry. For example, it is no longer obvious that swapping  $\xi$  with  $\eta$  swaps `bE` with `bG` — though that must still be the case:

`In[ ]:= Simplify[bEfullSimp - (bGfullSimp /. {ξ → η, η → ξ})]`

`Out[ ]:= 0`

---

## [A6]: The curvature $K$ of $(E_5, e_5)$

We compute the Gaussian curvature via the Brioschi formula (Alfred Gray [8], page 533):

$$\begin{aligned} \text{In}[*]:= \text{bKRaw} = & \left( \text{Det} \left[ \left\{ \left\{ -D[\text{bE}, \eta, \eta] / 2 + D[\text{bF}, \xi, \eta] - D[\text{bG}, \xi, \xi] / 2, \right. \right. \right. \\ & D[\text{bE}, \xi] / 2, D[\text{bF}, \xi] - D[\text{bE}, \eta] / 2 \}, \\ & \{ D[\text{bF}, \eta] - D[\text{bG}, \xi] / 2, \text{bE}, \text{bF} \}, \\ & \{ D[\text{bG}, \eta] / 2, \text{bF}, \text{bG} \} \} \right] - \\ & \text{Det} \left[ \left\{ \left\{ 0, D[\text{bE}, \eta] / 2, D[\text{bG}, \xi] / 2 \right\}, \right. \right. \\ & \{ D[\text{bE}, \eta] / 2, \text{bE}, \text{bF} \}, \\ & \left. \left. \{ D[\text{bG}, \xi] / 2, \text{bF}, \text{bG} \} \right\} \right] \right) / (\text{bE} \text{bG} - \text{bF}^2)^2; \end{aligned}$$

As in [A4], we replace the secants that differentiation has introduced with tangents and then FullSimplify without trigonometry.

$$\text{In}[*]:= \text{bK} = \text{FullSimplify}[\text{bKRaw} /. \text{secToTan}, \text{Trig} \rightarrow \text{False}]$$

$$\begin{aligned} \text{Out}[*]:= & - \left( \left( 25 \left( 1 + \tan\left[\frac{\eta}{2}\right]^2 \right)^2 \left( 1 + \tan\left[\frac{\xi}{2}\right]^2 \right)^2 \right. \right. \\ & \left( 825 + 375 \tan\left[\frac{\xi}{2}\right]^2 + 2355 \tan\left[\frac{\xi}{2}\right]^4 - 459 \tan\left[\frac{\xi}{2}\right]^6 + 17 \tan\left[\frac{\eta}{2}\right]^6 \left( -3 + \tan\left[\frac{\xi}{2}\right]^2 \right)^3 + \right. \\ & \tan\left[\frac{\eta}{2}\right]^4 \left( 2355 + 2109 \tan\left[\frac{\xi}{2}\right]^2 + 689 \tan\left[\frac{\xi}{2}\right]^4 - 153 \tan\left[\frac{\xi}{2}\right]^6 \right) + \\ & \left. \left. \tan\left[\frac{\eta}{2}\right]^2 \left( 375 - 3415 \tan\left[\frac{\xi}{2}\right]^2 + 2109 \tan\left[\frac{\xi}{2}\right]^4 + 459 \tan\left[\frac{\xi}{2}\right]^6 \right) \right) \right) / \right. \\ & \left( \tan\left[\frac{\eta}{2}\right]^6 \left( -3 + \tan\left[\frac{\xi}{2}\right]^2 \right)^3 - 3 \left( 25 + 75 \tan\left[\frac{\xi}{2}\right]^2 - 5 \tan\left[\frac{\xi}{2}\right]^4 + 9 \tan\left[\frac{\xi}{2}\right]^6 \right) - \right. \\ & \tan\left[\frac{\eta}{2}\right]^4 \left( -15 + 123 \tan\left[\frac{\xi}{2}\right]^2 + 83 \tan\left[\frac{\xi}{2}\right]^4 + 9 \tan\left[\frac{\xi}{2}\right]^6 \right) + \\ & \left. \left. \tan\left[\frac{\eta}{2}\right]^2 \left( -225 - 695 \tan\left[\frac{\xi}{2}\right]^2 - 123 \tan\left[\frac{\xi}{2}\right]^4 + 27 \tan\left[\frac{\xi}{2}\right]^6 \right) \right)^2 \right) \end{aligned}$$

Expressing  $K$  as a rational function of the Weierstrass variables, we get a quotient with 16-term factors of degree 12 in both numerator and denominator:

$$\text{In}[*]:= \text{bK} /. \text{halfAngleBackSubs} // \text{Factor}$$

$$\begin{aligned} \text{Out}[*]:= & - \left( \left( 25 (1 + x^2)^2 (1 + y^2)^2 \right. \right. \\ & (825 + 375 x^2 + 2355 x^4 - 459 x^6 + 375 y^2 - 3415 x^2 y^2 + 2109 x^4 y^2 + 459 x^6 y^2 + 2355 y^4 + \\ & 2109 x^2 y^4 + 689 x^4 y^4 - 153 x^6 y^4 - 459 y^6 + 459 x^2 y^6 - 153 x^4 y^6 + 17 x^6 y^6) \left. \right) / \\ & (-75 - 225 x^2 + 15 x^4 - 27 x^6 - 225 y^2 - 695 x^2 y^2 - 123 x^4 y^2 + 27 x^6 y^2 + 15 y^4 - \\ & 123 x^2 y^4 - 83 x^4 y^4 - 9 x^6 y^4 - 27 y^6 + 27 x^2 y^6 - 9 x^4 y^6 + x^6 y^6)^2 \end{aligned}$$

The extremes of curvature are at the  $\pi/4$  and  $\pi/5$  vertices:

$$\text{In}[*]:= \text{bK} /. \{ \xi \rightarrow 0, \eta \rightarrow 0 \}$$

$$\text{Out}[*]:= -\frac{11}{3}$$

$$\text{In}[*]:= \text{bK} /. \{ \xi \rightarrow 2\pi/5, \eta \rightarrow 2\pi/5 \} // \text{Simplify}$$

$$\text{Out}[*]:= -1$$

The curvature is intriguingly constant along the ditri-pentagon loops. We here consider three of them:

```
In[ ]:= bK /. {ξ → 2 π / 3} // Simplify
```

```
Out[ ]:= - 50
          21
```

```
In[ ]:= bK /. {η → π / 3 - ξ} // FullSimplify
```

```
Out[ ]:= - 50
          21
```

```
In[ ]:= bK /. {η → π / 3 + ξ} // FullSimplify
```

```
Out[ ]:= - 200 Cos[ 1/6 (π + 3 ξ) ]^2
          21 (2 + Cos[ξ] - √3 Sin[ξ])
```

Since FullSimplify didn't manage to simplify that third one unaided, we give a hint:

```
In[ ]:= (bK /. {η → π / 3 + ξ} // Simplify) /. Cos[arg_] ^ 2 → (1 + Cos[2 arg]) / 2 // Simplify
```

```
Out[ ]:= - 50
          21
```

## [A7]: The basics of solving the ODE in (9)

We here compute the isothermal coordinates depicted in the bottom images of Figures 12 and 14. This involves solving the differential equation in (9) using machine precision — that is, IEEE double-precision floating point.

Section 10.2 explains that, in some regions, we need a version of Sqrt in (9) that tracks the motion of the solution process along the two-sheeted Riemann surface of the square-root function, rather than just using the negative real axis as a fixed branch cut. To achieve this, the function memSqrt stores the last square root that it computed in the variable lastSqrt, which is dynamically bound by a Block in which the call to NDSolveValue occurs. For

Figure 12, we have the following code:

```
In[ ]:= memSqrt[z_ /; NumberQ[z]] := With[{s = Sqrt[z]},
      lastSqrt = If[Abs[lastSqrt + s] < Abs[lastSqrt - s], -s, s]]

In[ ]:= isoIEEE[{argξ_, argη_}] :=
  Block[{lastSqrt = 1},
    NDSolveValue[{
      q'[r] == ((-bF - I memSqrt[bE bG - bF^2]) / bE) /. {ξ → q[r], η → r},
      q[argη] == argξ,
      q, {r, 0, argη}][0]]
```

For Figure 14, the values  $E$ ,  $F$ , and  $G$  must be expressed in the rotated coordinate system  $(\mu, \nu)$ . We use a suffix of “r” to denote “in the rotated coordinates”.

$\text{In}[*]:= \text{bffffr} = \text{bfff} /. \{\xi \rightarrow (\mu - \nu) / 2, \eta \rightarrow (\mu + \nu) / 2\};$

$\text{In}[*]:= \text{bEr} = \text{FullSimplify}[\text{Coefficient}[\text{bffffr}, \text{Dt}[\mu]^2], \text{Trig} \rightarrow \text{False}]$

$$\begin{aligned} \text{Out}[*]= & - \left( \left( 150 + 335 \tan\left[\frac{\mu + \nu}{4}\right]^2 - 60 \tan\left[\frac{\mu + \nu}{4}\right]^4 + \right. \right. \\ & 27 \tan\left[\frac{\mu + \nu}{4}\right]^6 + 3 \tan\left[\frac{\mu - \nu}{4}\right]^6 \left( -3 + \tan\left[\frac{\mu + \nu}{4}\right]^2 \right)^2 + \\ & 4 \tan\left[\frac{\mu - \nu}{4}\right]^5 \tan\left[\frac{\mu + \nu}{4}\right] \left( -3 + \tan\left[\frac{\mu + \nu}{4}\right]^2 \right) \left( 9 + \tan\left[\frac{\mu + \nu}{4}\right]^2 \right) + \\ & 8 \tan\left[\frac{\mu - \nu}{4}\right]^3 \tan\left[\frac{\mu + \nu}{4}\right] \left( 5 + \tan\left[\frac{\mu + \nu}{4}\right]^2 \right) \left( -5 + 3 \tan\left[\frac{\mu + \nu}{4}\right]^2 \right) - \\ & 4 \tan\left[\frac{\mu - \nu}{4}\right] \tan\left[\frac{\mu + \nu}{4}\right] \left( 55 + 50 \tan\left[\frac{\mu + \nu}{4}\right]^2 + 27 \tan\left[\frac{\mu + \nu}{4}\right]^4 \right) + \\ & \tan\left[\frac{\mu - \nu}{4}\right]^2 \left( 335 + 980 \tan\left[\frac{\mu + \nu}{4}\right]^2 + 131 \tan\left[\frac{\mu + \nu}{4}\right]^4 - 18 \tan\left[\frac{\mu + \nu}{4}\right]^6 \right) + \\ & \left. \tan\left[\frac{\mu - \nu}{4}\right]^4 \left( -60 + 131 \tan\left[\frac{\mu + \nu}{4}\right]^2 + 18 \tan\left[\frac{\mu + \nu}{4}\right]^4 + 3 \tan\left[\frac{\mu + \nu}{4}\right]^6 \right) \right) / \\ & \left( 200 \left( \tan\left[\frac{\mu - \nu}{4}\right]^4 \left( -3 + \tan\left[\frac{\mu + \nu}{4}\right]^2 \right)^2 + \left( -3 + \tan\left[\frac{\mu + \nu}{4}\right]^2 \right) \left( 5 + 9 \tan\left[\frac{\mu + \nu}{4}\right]^2 \right) - \right. \right. \\ & \left. \left. 2 \tan\left[\frac{\mu - \nu}{4}\right]^2 \left( 11 + 30 \tan\left[\frac{\mu + \nu}{4}\right]^2 + 3 \tan\left[\frac{\mu + \nu}{4}\right]^4 \right) \right) \right) \right) \end{aligned}$$

$\text{In}[*]:= \text{bFr} = \text{FullSimplify}[\text{Coefficient}[\text{bffffr}, \text{Dt}[\mu] \text{Dt}[\nu]] / 2, \text{Trig} \rightarrow \text{False}]$

$$\begin{aligned} \text{Out}[*]= & \left( 3 \tan\left[\frac{\mu - \nu}{4}\right]^6 \left( -3 + \tan\left[\frac{\mu + \nu}{4}\right]^2 \right)^2 - \right. \\ & \tan\left[\frac{\mu + \nu}{4}\right]^2 \left( 115 + 30 \tan\left[\frac{\mu + \nu}{4}\right]^2 + 27 \tan\left[\frac{\mu + \nu}{4}\right]^4 \right) + \\ & \tan\left[\frac{\mu - \nu}{4}\right]^4 \left( 30 - 175 \tan\left[\frac{\mu + \nu}{4}\right]^2 - 3 \tan\left[\frac{\mu + \nu}{4}\right]^6 \right) + \\ & \left. \tan\left[\frac{\mu - \nu}{4}\right]^2 \left( 115 + 175 \tan\left[\frac{\mu + \nu}{4}\right]^4 + 18 \tan\left[\frac{\mu + \nu}{4}\right]^6 \right) \right) / \\ & \left( 200 \left( \tan\left[\frac{\mu - \nu}{4}\right]^4 \left( -3 + \tan\left[\frac{\mu + \nu}{4}\right]^2 \right)^2 + \left( -3 + \tan\left[\frac{\mu + \nu}{4}\right]^2 \right) \left( 5 + 9 \tan\left[\frac{\mu + \nu}{4}\right]^2 \right) - \right. \right. \\ & \left. \left. 2 \tan\left[\frac{\mu - \nu}{4}\right]^2 \left( 11 + 30 \tan\left[\frac{\mu + \nu}{4}\right]^2 + 3 \tan\left[\frac{\mu + \nu}{4}\right]^4 \right) \right) \right) \end{aligned}$$

`In[ ]:= bGr = FullSimplify[Coefficient[bfffr, Dt[v]^2], Trig → False]`

$$\begin{aligned} \text{Out[ ]}= & - \left( \left( 150 + 335 \tan\left[\frac{\mu + \nu}{4}\right]^2 - 60 \tan\left[\frac{\mu + \nu}{4}\right]^4 + \right. \right. \\ & 27 \tan\left[\frac{\mu + \nu}{4}\right]^6 + 3 \tan\left[\frac{\mu - \nu}{4}\right]^6 \left( -3 + \tan\left[\frac{\mu + \nu}{4}\right]^2 \right)^2 - \\ & 4 \tan\left[\frac{\mu - \nu}{4}\right]^5 \tan\left[\frac{\mu + \nu}{4}\right] \left( -3 + \tan\left[\frac{\mu + \nu}{4}\right]^2 \right) \left( 9 + \tan\left[\frac{\mu + \nu}{4}\right]^2 \right) - \\ & 8 \tan\left[\frac{\mu - \nu}{4}\right]^3 \tan\left[\frac{\mu + \nu}{4}\right] \left( 5 + \tan\left[\frac{\mu + \nu}{4}\right]^2 \right) \left( -5 + 3 \tan\left[\frac{\mu + \nu}{4}\right]^2 \right) + \\ & 4 \tan\left[\frac{\mu - \nu}{4}\right] \tan\left[\frac{\mu + \nu}{4}\right] \left( 55 + 50 \tan\left[\frac{\mu + \nu}{4}\right]^2 + 27 \tan\left[\frac{\mu + \nu}{4}\right]^4 \right) + \\ & \tan\left[\frac{\mu - \nu}{4}\right]^2 \left( 335 + 980 \tan\left[\frac{\mu + \nu}{4}\right]^2 + 131 \tan\left[\frac{\mu + \nu}{4}\right]^4 - 18 \tan\left[\frac{\mu + \nu}{4}\right]^6 \right) + \\ & \left. \tan\left[\frac{\mu - \nu}{4}\right]^4 \left( -60 + 131 \tan\left[\frac{\mu + \nu}{4}\right]^2 + 18 \tan\left[\frac{\mu + \nu}{4}\right]^4 + 3 \tan\left[\frac{\mu + \nu}{4}\right]^6 \right) \right) / \\ & \left( 200 \left( \tan\left[\frac{\mu - \nu}{4}\right]^4 \left( -3 + \tan\left[\frac{\mu + \nu}{4}\right]^2 \right)^2 + \left( -3 + \tan\left[\frac{\mu + \nu}{4}\right]^2 \right) \left( 5 + 9 \tan\left[\frac{\mu + \nu}{4}\right]^2 \right) - \right. \right. \\ & \left. \left. 2 \tan\left[\frac{\mu - \nu}{4}\right]^2 \left( 11 + 30 \tan\left[\frac{\mu + \nu}{4}\right]^2 + 3 \tan\left[\frac{\mu + \nu}{4}\right]^4 \right) \right) \right) \right) \end{aligned}$$

We could instead have computed bEr, bFr, and bGr as linear combinations of the unrotated bE, bF, and bG. Since the rotated variables  $\mu$  and  $\nu$  are related to the unrotated variables  $\xi$  and  $\eta$  by

$$\begin{pmatrix} \xi \\ \eta \end{pmatrix} = \begin{pmatrix} \frac{1}{2} & -\frac{1}{2} \\ \frac{1}{2} & \frac{1}{2} \end{pmatrix} \cdot \begin{pmatrix} \mu \\ \nu \end{pmatrix}$$

we have

$$\begin{pmatrix} \text{bEr} & \text{bFr} \\ \text{bFr} & \text{bGr} \end{pmatrix} = \begin{pmatrix} \frac{1}{2} & \frac{1}{2} \\ -\frac{1}{2} & \frac{1}{2} \end{pmatrix} \cdot \begin{pmatrix} \text{bE} & \text{bF} \\ \text{bF} & \text{bG} \end{pmatrix} \cdot \begin{pmatrix} \frac{1}{2} & -\frac{1}{2} \\ \frac{1}{2} & \frac{1}{2} \end{pmatrix} =$$

$$\begin{pmatrix} \frac{1}{4} (\text{bE} + 2 \text{bF} + \text{bG}) & \frac{1}{4} (-\text{bE} + \text{bG}) \\ \frac{1}{4} (-\text{bE} + \text{bG}) & \frac{1}{4} (\text{bE} - 2 \text{bF} + \text{bG}) \end{pmatrix}$$

And indeed, corresponding entries of the matrices on the left and the right are equal:

`In[ ]:= bEr - ((bE + 2 bF + bG) / 4) /. {ξ → (μ - ν) / 2, η → (μ + ν) / 2} // Simplify`

`Out[ ]:= 0`

`In[ ]:= bFr - ((-bE + bG) / 4) /. {ξ → (μ - ν) / 2, η → (μ + ν) / 2} // Simplify`

`Out[ ]:= 0`

`In[ ]:= bGr - ((bE - 2 bF + bG) / 4) /. {ξ → (μ - ν) / 2, η → (μ + ν) / 2} // Simplify`

`Out[ ]:= 0`

Given the rotated first fundamental form, the code for Figure 14 is no surprise:

```

In[ ]:= isoIEEEr[{argμ_, argv_}] :=
  Block[{lastSqrt = 1},
    NDSolveValue[{
      q'[r] == ((-bFr - I memSqrt[bEr bGr - bFr^2]) / bEr) /. {μ → q[r], ν → r},
      q[argν] == argμ},
      q, {r, 0, argν}][0]]

```

---

## [A8]: Approximating the function $h$

---

### Solving the ODE in (9) accurately

To approximate the analytic function  $h$  accurately, we first need to accurately compute the conformal tract  $T_{\text{cnf}}$  in the bottom image of Figure 14. And that requires solving the rotated version of the ODE in (9) accurately.

Along with IEEE doubles, Mathematica provides an arbitrary-precision floating point whose basic operations use *significance arithmetic*, a cheaper cousin of interval arithmetic, to bound the round-off errors that accumulate during easy stuff, such as arithmetic and the standard transcendental functions [18]. For sophisticated stuff, however, such as numerical integration or the numerical solution of differential equations, you specify a *PrecisionGoal* and an *AccuracyGoal*, goals for which you would like Mathematica to strive. You also specify the *WorkingPrecision* to be used during the calculation.

Mathematica uses *Accuracy* to mean absolute accuracy, while *Precision* means relative accuracy. Given goals for both, Mathematica strives to achieve the easier of the two goals. We set our *PrecisionGoal* to *Infinity*, which tells Mathematica to focus on our *AccuracyGoal*. Mathematica seems able to solve Gauss’s ODE in (9) to whatever accuracy we like, but convincing it to do so is a bit complicated. (The following code strives for high accuracy without worrying about the computation time.)

The function *isoGoal* tackles the first issue, which is setting the *WorkingPrecision*. If  $g$  is our *AccuracyGoal*, then setting the *WorkingPrecision* to  $g + 5$  is often adequate. But there are rare combinations of starting points and *WorkingPrecisions* that generate a warning message and an inaccurate result. The function *isoGoal*, if it detects such a warning, increments the *WorkingPrecision* by 5 and tries again. Also, for  $g > 10$ , *isoGoal* asks *NDSolveValue* to use the solution method “*StiffnessSwitching*”, which, experience reveals, generates many fewer warnings on these problems.

A fine point: Most of the warnings that *isoGoal* might detect warn of a possible inaccuracy in the output of *NDSolveValue*. But *NDSolveValue* also issues a warning — the warning *NDSolveValue::precw* — when it is passed input values whose precision is lower than the *WorkingPrecision*. In our situation, the coordinates  $s$  and  $t$  passed into *isoGoal* may well

have precision lower than some of the WorkingPrecisions that we adopt, looking for one that is free of output-related warnings. So we always ignore the input-related warning `NDSolveValue::precw`.

```
In[ ]:= isoGoal::novalidwp =
  "No warning-free value for the WorkingPrecision was found.";

isoGoal[{s_, t_}, g_] :=
  Catch[
    Do[Block[{lastSqrt = 1, res, q, r},
      Quiet[Check[Quiet[
        res = NDSolveValue[{
          q'[r] ==
            ((-bFr - I memSqrt[bEr bGr - bFr^2]) / bEr) /. {μ → q[r], ν → r},
          q[t] == s},
        q, {r, 0, t},
        AccuracyGoal → g, PrecisionGoal → Infinity,
        WorkingPrecision → wp,
        Method → If[g > 10, "StiffnessSwitching", Automatic]][0],
        {NDSolveValue::precw}],
        (* Always ignore that input-related warning. *)
        res = Indeterminate]]];
    (* Discard the result given any other warning. *)
    If[NumberQ[res], Throw[res]]],
    {wp, g + 5, 300, 5}];
  Message[isoGoal::novalidwp]
```

The actual accuracy of the value returned by `isoGoal` may fall short of the `AccuracyGoal` that we requested. With no independent source of accurate solutions to the ODE, we won't try for guaranteed accuracy. Instead, as an engineering compromise, the following function `isoCare` tries to do as well as `NDSolveValue` allows, aiming for a result whose absolute error is less than  $10^{-b}$ .

The function `isoCare` calls `isoGoal` for three different `AccuracyGoals`, of the form  $g$ ,  $g + 5$ , and  $g + 10$ . We expect the third result to be significantly more accurate than the first (although perhaps not 10 digits more accurate), with the second of intermediate accuracy. The function `isoCare` first checks that the gap between second and third is smaller than the gap between first and third, as we would expect. It then checks whether the gap between first and third is smaller than our hoped-for error bound of  $10^{-b}$ . If either of those tests fails, it increases  $g$  and tries again. If both tests succeed, it concludes that the third value is accurate enough for us, with an error less than  $10^{-b}$ . It returns that third value, telling Mathematica (via the function `N`) that its `Accuracy` is  $b$  — so that Mathematica can properly bound the errors of subsequent values that are computed from it.

```
In[ ]:= isoCare::accfail = "Could not solve ODE to requested accuracy.";
```

```

In[ ]:= isoCare[{s_, t_}, b_] :=
  Catch[
    Do[Block[{loAcc, mdAcc, hiAcc},
      loAcc = isoGoal[{s, t}, g];
      mdAcc = isoGoal[{s, t}, g + 5];
      hiAcc = isoGoal[{s, t}, g + 10];
      If[RealExponent[mdAcc - hiAcc] < RealExponent[loAcc - hiAcc] < -b ∨
        loAcc == mdAcc == hiAcc == 0, (* result exactly zero is also okay *)
        Throw[N[hiAcc, {Infinity, b}]]
      (* to examine the failing cases for debugging purposes, add here:
        Sow[{RealExponent[mdAcc - hiAcc], RealExponent[loAcc - hiAcc],
          loAcc, mdAcc, hiAcc}] *)
    ],
    {g, b + 1, 300, 5}];
  Message[isoCare::accfail]]

```

## The input triangle $H_{in}$

The analytic function  $h$  takes the input triangle  $H_{in}$  to the output triangle  $H_{out}$ , matching up their corresponding vertices. The triangle  $H_{in}$  is the conformal tract image  $T_{cnf}$  from the bottom of Figure 14, but shifted to the left to put the point  $M$ , the midpoint of its hypotenuse, at the origin. So the hypotenuse of  $H_{in}$  is the real axis, from  $-2\pi/5$  to  $+2\pi/5$ . To compute the short and long legs of  $H_{in}$  accurately, we first compute the short and long legs of  $T_{in}$  from Figure 1 symbolically; we then rotate them by  $\pi/4$  clockwise; we use `isoCare` to accurately solve the ODE in (9), getting the short and long legs of  $T_{cnf}$ ; and we finally shift leftward by subtracting the real number  $2\pi/5$  from the complex output of `isoCare`.

We parameterize the short leg from 0 to 1, from its  $\pi/4$  vertex to its  $\pi/2$  vertex; and we pass our target accuracy in as a second parameter.

```

In[ ]:= sleg[t_, b_] := With[{ξ = 0, η = t π / 3},
  isoCare[{η + ξ, η - ξ}, b] - 2 π / 5]

```

For the long leg, we need to do some trigonometry to trace the long leg of  $T_{in}$ . The convex pentagons along that long leg are mirror symmetric on a blue base, and projecting down onto that base reveals that  $1/2 + \cos[\eta] = \cos[\xi/2]$ . We parameterize the long leg by having  $\xi$  increase from 0 to 1 while moving from the  $\pi/2$  vertex to the  $\pi/5$  vertex. Given  $\xi$ , we then solve for  $\eta$  from that equation; but we treat the  $\pi/5$  vertex, where  $\xi = 2\pi/5$ , as a special case, in order to get the answer in that case, which is also  $2\pi/5$ , as an exact result:

```

In[ ]:= lleg[t_, b_] := With[{ξ = t 2 π / 5},
  With[{η = If[ξ == 2 π / 5, 2 π / 5, ArcCos[Cos[ξ / 2] - 1 / 2]]},
    isoCare[{η + ξ, η - ξ}, b] - 2 π / 5]

```

By the way, while the special square-root routine `memSqrt` is needed at various places in Figures 12 and 14, it isn't needed in Figure 14 when transforming the region  $T_{in}^{rot}$  into  $T_{cnf}$ . So we could here replace the `memSqrt` in `isoGoal` with Mathematica's standard `Sqrt`. We

don't bother to do so, since `memSqrt` imposes little overhead.

## The output triangle $H_{\text{out}}$

We choose, as our output triangle  $H_{\text{out}}$ , the (2,4,5)-triangle shown on the left in Figure 15, which has the center of the Poincaré disk as the midpoint of its hypotenuse. Let the Euclidean circle that extends the short leg of  $H_{\text{out}}$  be centered at  $\{\text{slcx}, \text{slcy}\}$  and have radius  $\text{slr}$ , while the circle that extends its long leg is centered at  $\{\text{llcx}, \text{llcy}\}$  and has radius  $\text{llr}$ . Denote its  $\pi/2$ ,  $\pi/4$ , and  $\pi/5$  vertices as  $v_2$ ,  $v_4$ , and  $v_5$ ; and let the coordinates of  $v_4$  and  $v_5$  be  $\{-\text{halfhyp}, 0\}$  and  $\{\text{halfhyp}, 0\}$ . We have seven equations in seven unknowns. Solve can handle this system, but it takes a few minutes, so the code here is guarded by the Boolean flag `solveForHOut`.

```
In[*]:= solveForHOut = False;

In[*]:= If[solveForHOut, Solve[{
  (slcx + halfhyp)^2 + slcy^2 == slr^2, (* vertex v4 lies on the short leg *)
  (llcx - halfhyp)^2 + llcy^2 == llr^2, (* v5 lies on the long leg *)
  llcx^2 + llcy^2 == llr^2 + 1,
  (* long-leg circle is orthogonal to the absolute *)
  slcx^2 + slcy^2 == slr^2 + 1, (* short-
    leg circle is orthogonal to the absolute *)
  slr^2 + llr^2 == (slcx - llcx)^2 + (slcy - llcy)^2,
  (* angle at v2 is  $\pi/2$  *)
  slcy == -(halfhyp + slcx), (* angle at v4 is  $\pi/4$  *)
  llcy == Sqrt[1 + 2/Sqrt[5]] (llcx - halfhyp), (* angle at v5 is  $\pi/5$  *)
  slcx < 0, llcx > 0, slcy > 0, llcy > 0, slr > 0, llr > 0, halfhyp > 0},
  {slcx, slcy, slr, llcx, llcy, llr, halfhyp}, Reals] // FullSimplify //
  ToRadicals // First ]
```

$$\begin{aligned}
In[ ]:= \text{hOut} = \{ & \text{slcx} \rightarrow -\sqrt{1+\sqrt{5}+\sqrt{5+2\sqrt{5}}}, \text{slcy} \rightarrow \sqrt{\sqrt{5}+\sqrt{5+2\sqrt{5}}}, \\
& \text{slr} \rightarrow \sqrt{2\left(\sqrt{5}+\sqrt{5+2\sqrt{5}}\right)}, \\
& \text{llcx} \rightarrow \sqrt{1+\sqrt{5}+\sqrt{5+2\sqrt{5}}}, \text{llcy} \rightarrow \sqrt{2+\sqrt{5}+\sqrt{17+\frac{38}{\sqrt{5}}}}, \\
& \text{llr} \rightarrow \sqrt{2\left(1+\sqrt{5}+\sqrt{10+\frac{22}{\sqrt{5}}}\right)}, \\
& \text{halfhyp} \rightarrow \frac{-\sqrt{5+2\sqrt{5}+\sqrt{5(5+2\sqrt{5})}} + \sqrt{5+2\sqrt{5}+\sqrt{50+22\sqrt{5}}}}{(5+2\sqrt{5})^{1/4}} \};
\end{aligned}$$

It's not clear why Mathematica comes up with that complicated expression for halfhyp. We stipulated that halfhyp == -slcx - slcy, and that gives us a simpler formula:

$$\begin{aligned}
In[ ]:= \text{hOut}[[7]] = \text{halfhyp} \rightarrow (-\text{slcx} - \text{slcy}) /. \text{hOut} \\
Out[ ]:= \text{halfhyp} \rightarrow -\sqrt{\sqrt{5}+\sqrt{5+2\sqrt{5}}} + \sqrt{1+\sqrt{5}+\sqrt{5+2\sqrt{5}}}
\end{aligned}$$

We don't need the coordinates of the vertex v2, but here is a pair of valid formulas — one of many choices:

$$\begin{aligned}
In[ ]:= \{ & \text{v2x} \rightarrow \left( -\sqrt{2/\sqrt{5}} + 2\sqrt{-13-5\sqrt{5}+\sqrt{298+662/\sqrt{5}}} \right) / \\
& \left( -1-2\sqrt{5}+\sqrt{29+62/\sqrt{5}} \right), \\
& \text{v2y} \rightarrow \left( -2\sqrt{2(1+\sqrt{5})} + \sqrt{6+4\sqrt{5}+2\sqrt{29+62/\sqrt{5}}} \right) / \\
& \left( -1-2\sqrt{5}+\sqrt{29+62/\sqrt{5}} \right) \};
\end{aligned}$$

## Appealing to nonlinear least squares

For various degrees, we now search for a univariate polynomial  $C_{\text{deg}}$  of a complex variable with real coefficients that approximately maps  $H_{\text{in}}$  to  $H_{\text{out}}$ .

As Section 11.1 explains, there is no straightforward way to determine the actual max error of a candidate polynomial. Instead, we rate a candidate  $C$  by its maximal deviation, the maximal distance by which the short and long legs of the boundary of  $C(H_{\text{in}})$  stray either inside or outside of the corresponding boundary arcs of  $H_{\text{out}}$ . We refer to that deviation here as “radial error”, since we are comparing the distance to the center of the relevant circular arc with the radius of that arc. For convenience, we measure our radial errors using Euclidean distance in the Poincaré disk.

```
In[ ]:= radErr[z_, {a_, b_, r_}] :=
  (* comparing z to the circle with center {a,b} and radius r *)
  (Sqrt[(a - ComplexExpand[Re[z]])^2 + (b - ComplexExpand[Im[z]])^2] - r)
```

This argument  $z$  may be a value of the polynomial  $C_{\text{deg}}$ , expressed in terms of its unknown coefficients  $c[k]$ ; these calls to `ComplexExpand` tell Mathematica that those coefficients  $c[k]$  are real numbers, as we insist.

```
In[ ]:= slegRadErr[z_] := radErr[z, {slcx, slcy, slr}] /. hOut]
```

```
In[ ]:= llegRadErr[z_] := radErr[z, {llcx, llcy, llr}] /. hOut]
```

```
In[ ]:= chebSamp[k_, m_] :=
  (* the k'th of m+1 Chebyshev-distributed points in [0..1] *)
  (1 - Cos[k Pi / m]) / 2
```

The call `polyApprox[deg]` finds an approximating polynomial  $C_{\text{deg}}$  of degree `deg`. Experience reveals that we can typically get the radii of our approximated short and long legs accurate to about  $0.42 \text{ deg} + 3$  decimal digits. To retain a few significant digits in our computed errors, we set `acc` to  $0.42 \text{ deg} + 7$ . We compute the short and long legs of the input triangle  $H_{\text{in}}$  to that accuracy, and we evaluate our approximating polynomial to that accuracy.

We test the accuracy of our approximant at a dense set of test points. Our approximant will exploit the degrees of freedom in its coefficients to interpolate the desired radii at about `deg` points, distributed over the short and long legs; so there will be roughly `deg/2` humps in the error curve along each leg, alternating positive and negative. We allocate about ten test points to each such hump, putting  $5 \text{ deg} + 5$  test points along each leg. Since the humps of error get narrower near the ends of the legs, we Chebyshev-distribute our test points.

We search for the approximating polynomial using nonlinear least squares, which Mathematica provides via the function `FindMinimum`. The error metric that we try to minimize is the sum of the squared errors at a set of sample points along each leg. The precise number of such sample points isn't critical, though it is important that they be Chebyshev-distributed along each leg, to prevent the error from shooting up near the ends of the legs. Putting  $\text{deg} + 1$  sample points along each leg gives us twice as many constraints as variables, which works fine.

We represent our unknown polynomial in the monomial basis, whose numerical condition is known to be lousy; so we may have to set the `WorkingPrecision` used by `FindMinimum` quite high. On the other hand, we evaluate  $C_{\text{deg}}$  only at points along the short and long legs of  $H_{\text{in}}$ , and those points all have norms in the open interval  $(0.74 \dots 1.26)$  — and hence close to 1; that should help. Setting this `WorkingPrecision` to 2 acc turns out to be adequate, at least out through degree 250. (It's easy to tell if this `WorkingPrecision` has been set too low, since the resulting error curves then don't come anywhere near equioscillating.)

Our variables are the unknown coefficients  $c[0]$  through  $c[\text{deg}]$ . We initialize  $c[0]$  and  $c[1]$  to reasonable values, but we initialize all of the others to zero, letting the least-squares process figure them out. Once `FindMinimum` has computed them, we reduce their `Precision` to only acc, which should suffice for computing the values of the polynomial  $C_{\text{deg}}$  with Accuracy roughly acc.

The function `polyApprox` returns an association that gives the degree `deg`, the coefficients of  $C_{\text{deg}}$ , the max absolute radial error found at our test points, and, for plotting purposes, tables with the actual radial errors at the test points.

```

In[ ]:= polyApprox[deg_] := Module[{
  acc = Ceiling[0.42 deg + 7], testCnt = 5 deg + 5,
  sampCnt = deg,
  coeffs, unkPoly, metric, varList,
  foundMin, minPoly, minCoeffs,
  slegRadErrs, llegRadErrs},
  coeffs = Table[c[k], {k, 0, deg}];
  (* We use Fold to compute unkPoly with Horner's-rule nesting. *)
  unkPoly[z_] = Fold[z #1 + #2 &, 0, Table[c[deg - k], {k, 0, deg}]];
  metric =
  Sum[
    slegRadErr[unkPoly[sleg[chebSamp[k, sampCnt], acc]]]^2, {k, 0, sampCnt}] +
    Sum[llegRadErr[unkPoly[lleg[chebSamp[k, sampCnt], acc]]]^2,
      {k, 0, sampCnt}];
  varList = Join[{c[0], 1/1000}, {c[1], 167/1000}],
    Table[{c[k], 0}, {k, 2, deg}];
  foundMin = Quiet[FindMinimum[metric, varList,
    WorkingPrecision → 2 acc], {FindMinimum::precw}];
  (* Since the WorkingPrecision of FindMinimum is 2 acc,
  FindMinimum will warn us
  that our metric has accuracy only acc; we turn off that warning. *)
  minCoeffs = Table[c[k] → N[c[k] /. foundMin[[2]], acc], {k, 0, deg}];
  minPoly[z_] = unkPoly[z] /. minCoeffs;
  slegRadErrs = Table[{chebSamp[k, testCnt], slegRadErr[minPoly[
    sleg[chebSamp[k, testCnt], acc]]]}, {k, 0, testCnt}];
  llegRadErrs = Table[{chebSamp[k, testCnt], llegRadErr[minPoly[
    lleg[chebSamp[k, testCnt], acc]]]}, {k, 0, testCnt}];
  <| degree → deg,
  coeffVals → minCoeffs,
  maxLogErr →
    Max[Map[Composition[RealExponent, Last], Join[slegRadErrs, llegRadErrs]]],
  maxAbsErr → Max[Map[Composition[Abs, Last],
    Join[slegRadErrs, llegRadErrs]]],
  slegErrs → N[slegRadErrs],
  llegErrs → N[llegRadErrs] |>
]

```

I evaluated `polyApprox[deg]` for each `deg` in the following sequence:

```

In[ ]:= degSeq =
  Union[Range[1, 25], Range[25, 50, 5], Range[50, 100, 10], Range[100, 250, 25]]
Out[ ]:= {1, 2, 3, 4, 5, 6, 7, 8, 9, 10, 11, 12, 13, 14, 15, 16, 17, 18, 19, 20, 21, 22, 23,
  24, 25, 30, 35, 40, 45, 50, 60, 70, 80, 90, 100, 125, 150, 175, 200, 225, 250}

```

Since the last few of those calls took many hours to compute, we here simply read in the results from the data file `ApproximatingPolynomials.m`, where I saved them. (We assume that file is available in the same directory from which this notebook file, “`EquilateralPentagonMap.nb`”, was read.) After reading that data file, the value `poly[deg]` will be the association that I computed via the call `polyApprox[deg]`.

The call `polyApprox[250]` took about 95 hours on my Windows PC, by the way. Computing the sample points and doing the nonlinear least squares took the first 30 of those, while

computing the errors at the test points took the rest. The call `polyApprox[225]` took just 40 hours, and the times went down quickly from there.

```
In[ ]:= SetDirectory[NotebookDirectory[]];
```

```
In[ ]:= << "ApproximatingPolynomials.m";
```

Before doing anything else, let's check the precision of our computed errors, to verify that setting `acc = 0.42 deg + 7` was setting it high enough:

```
In[ ]:= DiscretePlot[Precision[Lookup[poly[deg], maxAbsErr]], {deg, degSeq}]
```

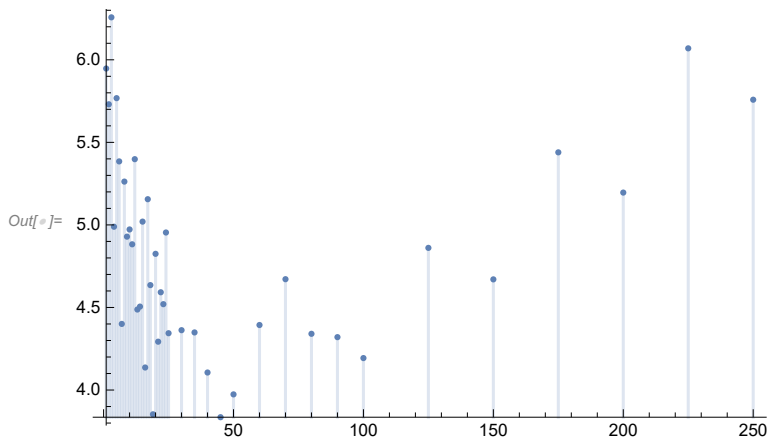

So we have roughly five digits of precision in our computed errors, which is plenty. (Indeed, it seems that setting `acc = 0.41 deg + 7` would have been adequate.) It is Mathematica's use of significance arithmetic [18], by the way, that allows us here to get good bounds on the precision of our computed errors.

How does the max radial error of  $C_{\text{deg}}$  vary with the degree?

```
In[ ]:= convPlot = ListPlot[Table[{d, Lookup[poly[d], maxLogErr]}], {d, degSeq}]]
```

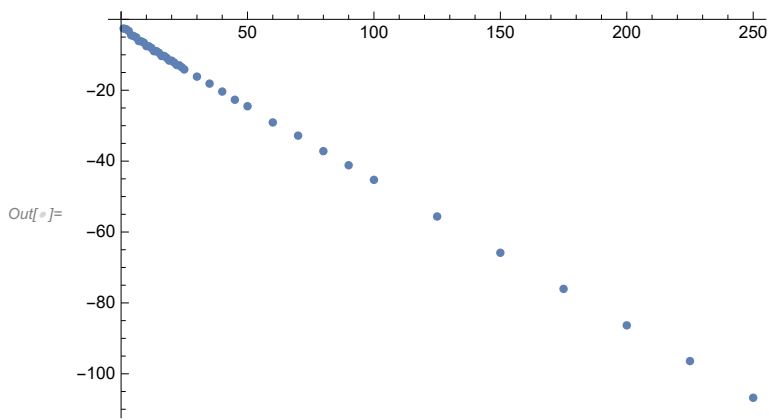

So the eventual convergence seems to be geometric. Fitting a line to the last five data points gives us:

```
In[ ]:= convFit = Fit[Table[{d, Lookup[poly[d], maxLogErr]}], {d, 150, 250, 25}], {1, t}, t]
```

```
Out[ ]:= -4.52804 - 0.408767 t
```

```
In[ ]:= Show[convPlot, Plot[convFit, {t, 0, 250}]]
```

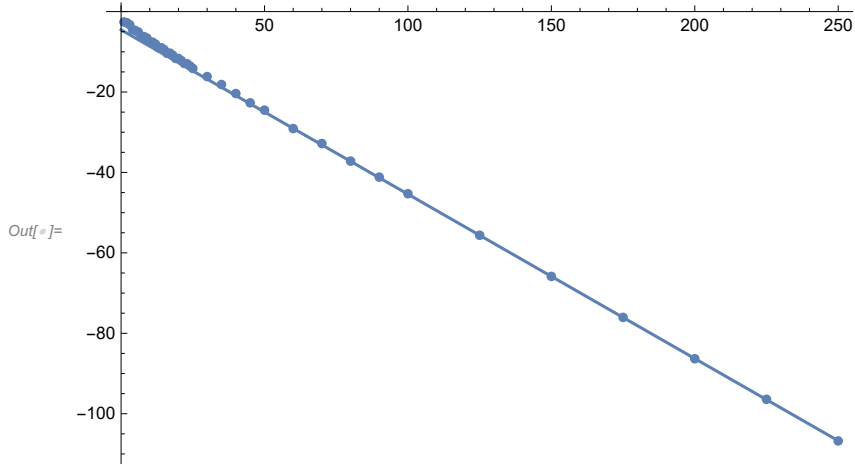

```
In[ ]:= 10^(-Coefficient[convFit, t, 1])
```

```
Out[ ]:= 2.56311
```

So a unit increase in the degree reduces the radial error by a factor of about 2.56. When the degree is small, a unit increase does a bit better than that; and there is a clear period-3 oscillation in the results:

```
In[ ]:= Show[ListPlot[Drop[Table[{d, Lookup[poly[d], maxLogErr]}], {d, degSeq}], -16]],  
Plot[convFit, {t, 0, 250}]]
```

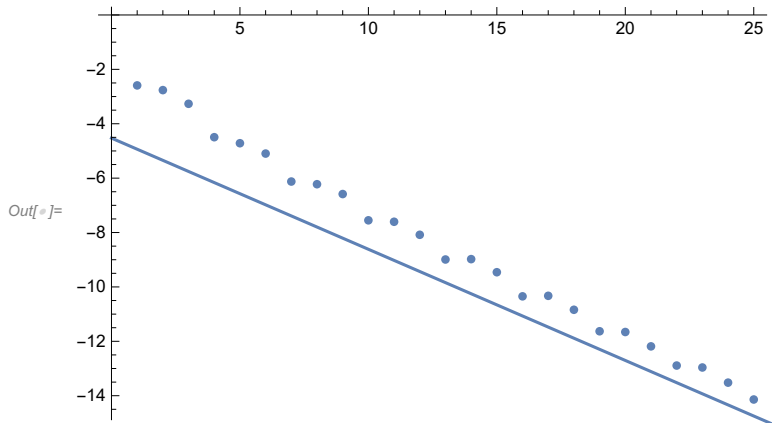

A period-3 oscillation appears also in the coefficients of the approximating polynomials. For example, here is a semilog plot of the coefficients of  $C_{50}$ , with the negative coefficients plotted as red dots, the positive as blue dots:

```
In[ ]:= c50[k_] := c[k] /. Lookup[poly[50], coeffVals]
```

```
In[ ]:= ListPlot[
  Table[Style[{k, Log[10, Abs[c50[k]]]}, If[c50[k] > 0, Blue, Red]], {k, 0, 50}]]
```

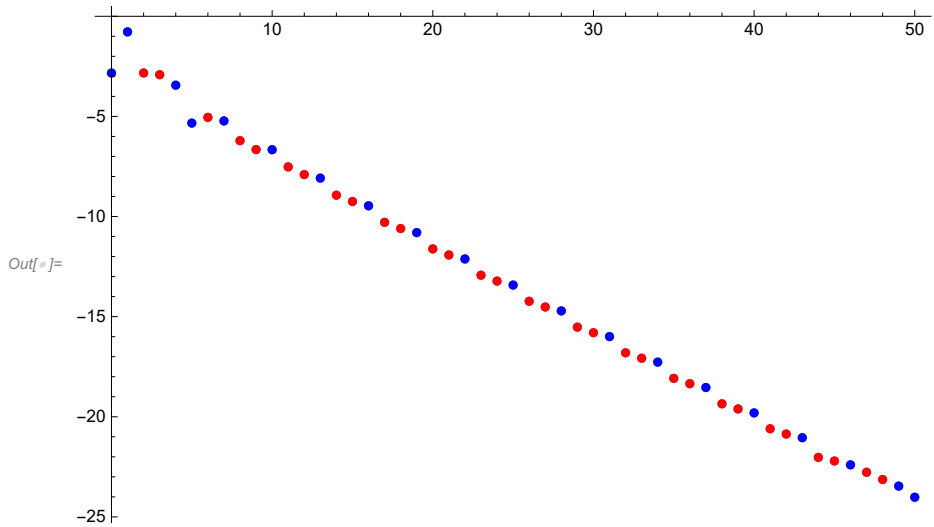

As Section 11.3 discusses, both of these period-3 oscillations arise because, when the analytic function  $h$  is expanded in a Taylor series at the point  $M$ , its convergence-limiting singularities, at  $Y$  and  $\bar{Y}$ , have phase roughly  $\pm 2\pi/3$ .

The radial-error functions pass through zero about  $\deg$  times overall, when we combine the short and long legs; and they come reasonably close to equioscillating. In the following sample plots, the radial errors for the short leg appear above those for the long leg, each plotted from its left to its right:

```
In[ ]:= errs[d_] := Column[{ListPlot[Lookup[poly[d], slegErrs], Joined → True,
  AspectRatio → 1/4, ImageSize → Large],
  ListPlot[Lookup[poly[d], llegErrs], Joined → True,
  AspectRatio → 1/4, ImageSize → Large]}]
```

In[ ]:= errs[10]

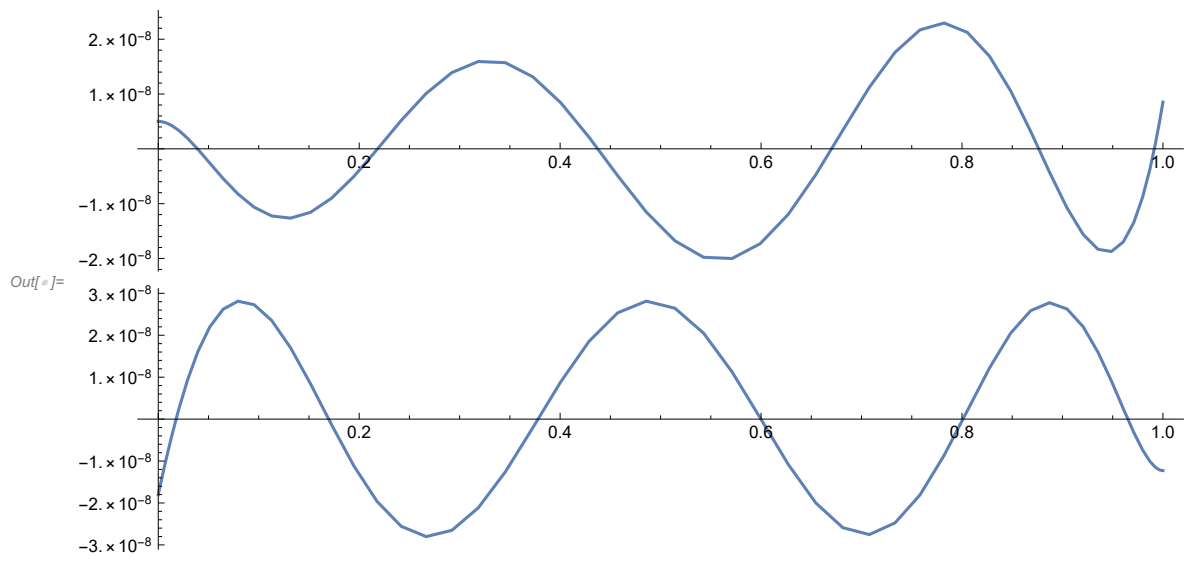

In[ ]:= errs[50]

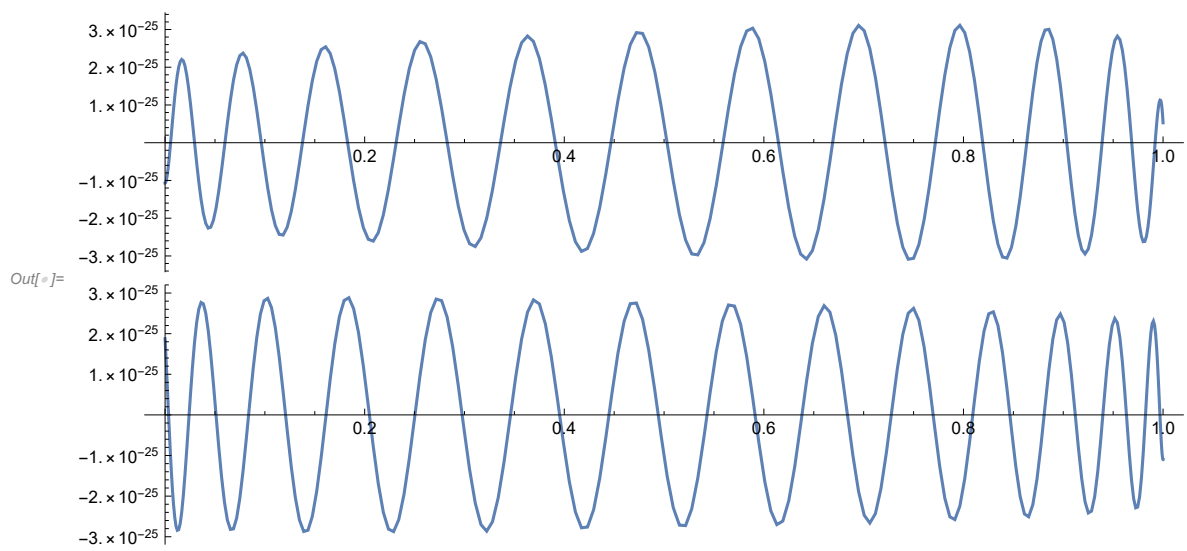

In[ ]:= **errs[100]**

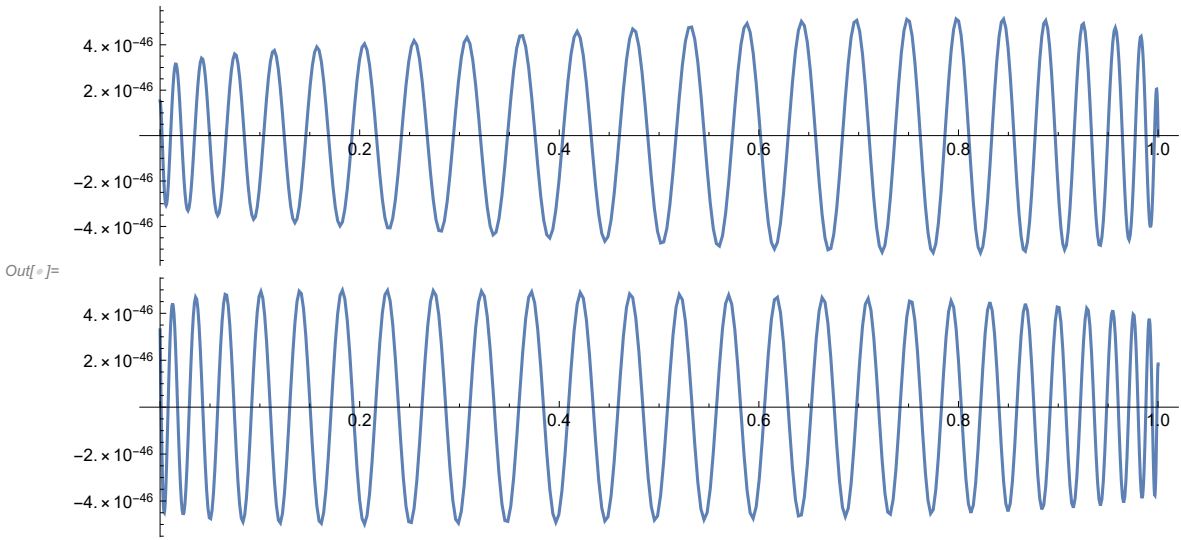

In[ ]:= **errs[250]**

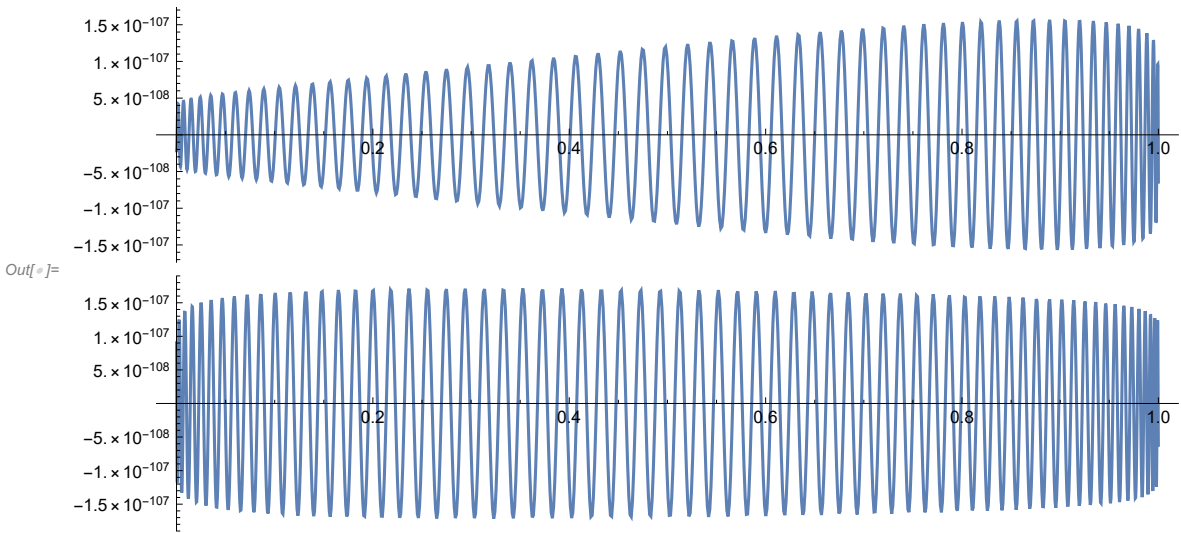

## [A9]: The procedure PoincareCoordinates

In this section, we implement, as a takeaway, a procedure named `PoincareCoordinates` that maps the region  $T_{\text{in}}$  in Figure 1 to the region  $T_{\text{out}}$  in Figure 2, with any requested accuracy, up to 100 digits. The mapping `PoincareCoordinates` happens in five steps, three easy steps alternating with two hard ones:

$T_{\text{in}} \rightarrow T_{\text{in}}^{\text{rot}}$ : We rotate the input region  $T_{\text{in}}$  clockwise  $\pi/4$  by setting  $\{\mu, \nu\} = \{\eta + \xi, \eta - \xi\}$ , thus putting its hypotenuse along the x-axis.

$T_{\text{in}}^{\text{rot}} \rightarrow T_{\text{cnf}}$ : By accurately solving the ODE (9) as in [A8], we alter the coordinates to be

isothermal as we move away from the x-axis, which is held pointwise fixed. This gives us the conformal tract image  $T_{\text{cnf}}$  shown at the bottom of Figure 14.

$T_{\text{cnf}} \rightarrow H_{\text{in}}$ : We shift  $T_{\text{cnf}}$  leftward in the complex plane, subtracting  $2\pi/5$  from the real part to put the midpoint  $M$  of its hypotenuse at the origin.

$H_{\text{in}} \rightarrow H_{\text{out}}$ : We conformally map  $H_{\text{in}}$  to the  $(2, 4, 5)$ -triangle  $H_{\text{out}}$  in Figure 15, using a precomputed univariate polynomial of a complex variable of some appropriate degree.

$H_{\text{out}} \rightarrow T_{\text{out}}$ : An orientation-preserving isometry of the hyperbolic plane then maps the triangle  $H_{\text{out}}$  to the output region  $T_{\text{out}}$ .

## The input region $T_{\text{in}}$

When the five edge vectors of an equilateral pentagon are drawn all leaving the origin, they partition the neighborhood of the origin into five angular sectors whose widths are nonnegative and sum to  $2\pi$ . You specify your pentagon of interest to PoincareCoordinates by giving the pair  $\{\xi, \eta\}$ , where  $\xi$  is the smallest and  $\eta$ , the second-smallest of those five sector widths. The pair  $\{\xi, \eta\}$  lies in the tract  $T_{\text{in}}$ , shown here and in Figure 1:

```
In[ ]:= T_in = Show[ContourPlot[0 == 1, {x, 0, 75}, {y, 0, 75},
  FrameTicks -> {Range[0, 72, 12], Range[0, 72, 12]}, FrameTicksStyle -> 14,
  FrameLabel -> {ξ, η}, RotateLabel -> False, LabelStyle -> 20],
  ContourPlot[x == 0, {x, -0.1, 72}, {y, 0, 60}],
  ContourPlot[y == x, {x, 0, 72}, {y, 0, 72}],
  ContourPlot[Cos[x Degree / 2] == 1 / 2 + Cos[y Degree], {x, 0, 72}, {y, 0, 72}]]
```

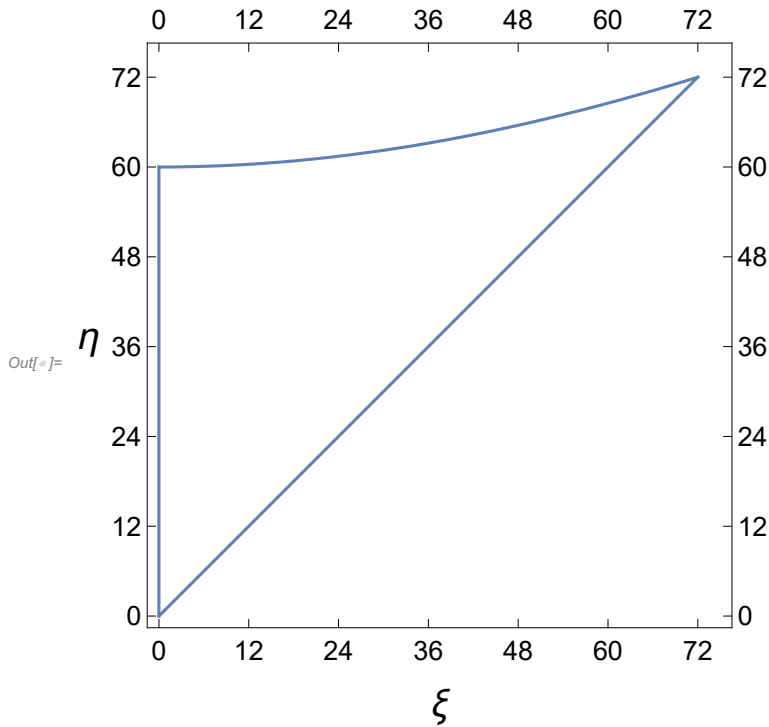

Along the short leg of a tract, the narrowest sector has width zero, so  $\xi = 0$ . Along the hypotenuse, the two narrowest sectors are tied for width, those widths being  $\xi$  and  $\eta$ , so  $\xi = \eta$ . Along the long leg, the two widest sectors are tied for width. The cluster of five edge vectors is then mirror symmetric across the one vector that doesn't bound either of those widest sectors, and projecting orthogonally onto that line of symmetry reveals that  $\text{Cos}[\xi/2] == 1/2 + \text{Cos}[\eta]$ , as we commented back in [A8].

There are two tracts that underlie  $T_{\text{in}}$ , one on each sheet. The sheet on which your particular pentagon lies is determined by the cyclic order of three things: its narrowest sector, its second-narrowest sector, and its one edge that doesn't bound either of those sectors. But that cyclic order doesn't affect the Poincaré coordinates of the point where your pentagon should be plotted.

## The output region $T_{\text{out}}$

We map  $T_{\text{in}}$  to the region labeled  $T_{\text{out}}$  in Figure 2. Here is  $T_{\text{out}}$  as a subset of the Poincaré disk:

```
In[ ]:= Graphics[{Circle[], Line[{{0, -1}, {0, 1}}],
  Line[{{-1, -1}/Sqrt[2], {1, 1}/Sqrt[2]}],
  Circle[{0, Sqrt[2 + Sqrt[5]]}, Sqrt[1 + Sqrt[5]]],
  {ArcTan[Sqrt[1 + Sqrt[5]]] - Pi, -ArcTan[Sqrt[1 + Sqrt[5]]]}]}
```

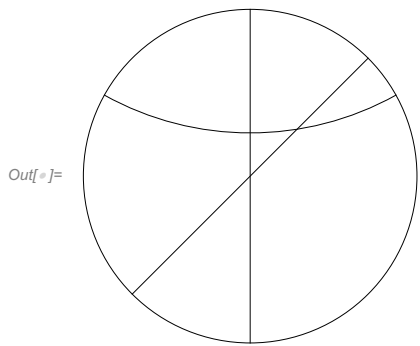

We don't need to compute the geometry of  $T_{\text{out}}$  in order to implement the function PoincareCoordinates. But let's compute it anyway, since it will come in handy for checking our answers.

We compute the center and radius of the Euclidean circle that forms the long leg of  $T_{\text{out}}$  as follows. Let that circle be centered at  $(0, y)$ , have radius  $r$ , and intersect the main diagonal

at  $(d, d)$ . Since  $45^\circ - 36^\circ == 9^\circ$  and since  $\text{Sin}[9^\circ] == \frac{1}{2} \sqrt{2 - \sqrt{\frac{1}{2} (5 + \sqrt{5})}}$  (a fact

not at Mathematica's fingertips), we then have:

```

In[ ]:= Solve[{
  1 + r^2 == y^2, (* long-leg circle is orthogonal to the absolute *)
  d^2 + (y - d)^2 == r^2, (* the  $\pi/5$  vertex lies on the long leg *)

  d/r ==  $\frac{1}{2} \sqrt{2 - \sqrt{\frac{1}{2}(5 + \sqrt{5})}}$ , (* angle at  $\pi/5$  vertex is  $36^\circ == \pi/5$  *)

  r > 0, y > 0}, {r, y, d}, Reals] // FullSimplify
Out[ ]:= {{r ->  $\sqrt{1 + \sqrt{5}}$ , y ->  $\sqrt{2 + \sqrt{5}}$ , d ->  $\frac{1}{2}(-5^{1/4} + \sqrt{2 + \sqrt{5}})$ }}

```

Thus, the  $\pi/2 = 90^\circ$  vertex of  $T_{\text{out}}$  has coordinates

$\{0, \sqrt{2 + \sqrt{5}} - \sqrt{1 + \sqrt{5}}\} \approx \{0, 0.2593\}$ , and its  $\pi/5 = 36^\circ$  vertex is at  $\{p, q\}$  where

$$p = q = \frac{1}{2} \left( -5^{1/4} + \sqrt{2 + \sqrt{5}} \right) \approx 0.2814.$$

```

In[ ]:= T_out = Show[ContourPlot[0 == 1, {p, 0, 0.3}, {q, 0, 0.3}],
  ContourPlot[p == 0, {p, -0.01, 0.3},
    {q, 0, Sqrt[2 + Sqrt[5]] - Sqrt[1 + Sqrt[5]]}],
  ContourPlot[p == q, {p, 0, 0.3}, {q, 0, (Sqrt[2 + Sqrt[5]] - 5^(1/4))/2}],
  ContourPlot[p^2 + (Sqrt[2 + Sqrt[5]] - q)^2 == 1 + Sqrt[5],
    {p, 0, (Sqrt[2 + Sqrt[5]] - 5^(1/4))/2}, {q, 0, 0.3}]]

```

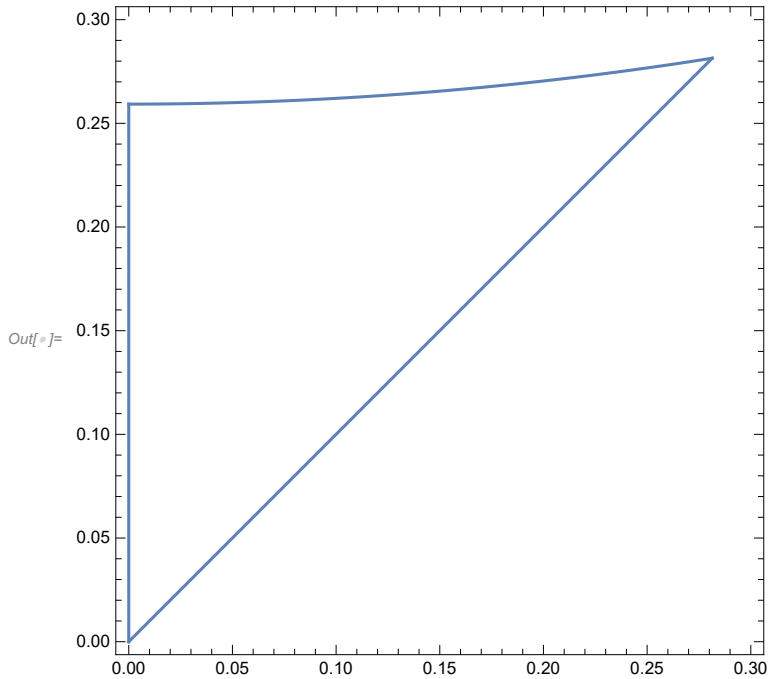

While  $T_{\text{in}}$  and  $T_{\text{out}}$  resemble each other, their shapes do differ. For one thing, the northeast vertex of  $T_{\text{in}}$  has an angle of only  $\text{ArcTan}[5 - 2\sqrt{5}] \approx 27.8^\circ$ , noticeably more acute than the  $36^\circ$  of  $T_{\text{out}}$ .

## Other output regions

A client of `PoincareCoordinates` may well want to plot their pentagon in some (2,4,5)-triangle other than  $T_{\text{out}}$ . It is up to them to deal with that issue, but here are some hints.

Every (2,4,5)-triangle is the image of  $T_{\text{out}}$  under an isometry of the hyperbolic plane. In the Poincaré-disk model, an isometry of the hyperbolic plane that preserves orientation maps the complex number  $z = p + i q$  to  $\frac{e^{i\varphi}(z-\alpha)}{1-\alpha^* z}$ , for some real angle  $\varphi$  and some complex number  $\alpha$  with  $\text{Abs}[\alpha] < 1$ . The point  $\alpha$  in the Poincaré disk models the point in the hyperbolic plane that maps to the origin under that isometry.

Any isometry that reverses orientation can be implemented by first reflecting  $T_{\text{out}}$  and then mapping that reflected result through an isometry that preserves orientation. (The map  $\{p, q\} \mapsto \{-p, q\}$  reflects  $T_{\text{out}}$  across its short leg, while  $\{p, q\} \mapsto \{q, p\}$  reflects it across its hypotenuse.)

## The code

We now give the code in the file “`EquilateralPentagonMap.m`”. It implements the routine `PoincareCoordinates`, distilling the above into a small package — well, small if we don’t charge for the data file `ApproximatingPolynomials.m`.

```
In[ ]:= (* :Title:
EquilateralPentagonMap.m -- a conformal map of the equilateral pentagons *)

In[ ]:= (* :Author: Lyle Ramshaw *)

In[ ]:= (* :Mathematica Version: 11.3 *)

In[ ]:= BeginPackage["EquilateralPentagonMap`"]

Out[ ]:= EquilateralPentagonMap`
```

```
PoincareCoordinates::usage =
"PoincareCoordinates[{ξ,η}, acc] takes an equilateral pentagon
and returns the Poincaré coordinates of the point, within a
(2,4,5)-triangle of a hyperbolic map, where that pentagon should
be plotted, accurate to 10^(-acc). The angles ξ and η are,
out of the ten pairs of edge vectors of the pentagon, the two
smallest nonnegative phase differences, measured in radians.";
```

```
In[ ]:= Begin["`Private`"]
```

```
Out[ ]:= EquilateralPentagonMap`Private`
```

We computed everything from first principles above; but this package doesn't need to redo that calculation. We here start with the formulas for  $E$ ,  $F$ , and  $G$  from (8), written as functions of the Weierstrass transforms  $x$  and  $y$ .

```
In[ ]:= bExy = - ((75 + 225 x^2 - 15 x^4 + 27 x^6 + 110 y^2 +  
490 x^2 y^2 - 22 x^4 y^2 - 18 x^6 y^2 - 45 y^4 + 153 x^2 y^4 + 9 x^4 y^4 + 3 x^6 y^4) /  
(50 (-15 - 22 x^2 + 9 x^4 - 22 y^2 - 60 x^2 y^2 - 6 x^4 y^2 + 9 y^4 - 6 x^2 y^4 + x^4 y^4))) ;
```

```
In[ ]:= bFxy = - ((x y (-55 - 50 x^2 - 27 x^4 - 50 y^2 + 20 x^2 y^2 + 6 x^4 y^2 - 27 y^4 + 6 x^2 y^4 + x^4 y^4) ) /  
(25 (-15 - 22 x^2 + 9 x^4 - 22 y^2 - 60 x^2 y^2 - 6 x^4 y^2 + 9 y^4 - 6 x^2 y^4 + x^4 y^4))) ;
```

```
In[ ]:= bGxy = - ((75 + 110 x^2 - 45 x^4 + 225 y^2 + 490 x^2 y^2 +  
153 x^4 y^2 - 15 y^4 - 22 x^2 y^4 + 9 x^4 y^4 + 27 y^6 - 18 x^2 y^6 + 3 x^4 y^6) /  
(50 (-15 - 22 x^2 + 9 x^4 - 22 y^2 - 60 x^2 y^2 - 6 x^4 y^2 + 9 y^4 - 6 x^2 y^4 + x^4 y^4))) ;
```

We convert to rotated coordinates using the linear combinations discussed in [A7], expressing the results in terms of the rotated variables  $\mu$  and  $\nu$ :

```
In[ ]:= bEr = ((bExy + 2 bFxy + bGxy) / 4) /. {x -> Tan[(μ - ν) / 4], y -> Tan[(μ + ν) / 4]} ;
```

```
In[ ]:= bFr = ((-bExy + bGxy) / 4) /. {x -> Tan[(μ - ν) / 4], y -> Tan[(μ + ν) / 4]} ;
```

```
In[ ]:= bGr = ((bExy - 2 bFxy + bGxy) / 4) /. {x -> Tan[(μ - ν) / 4], y -> Tan[(μ + ν) / 4]} ;
```

We next solve Gauss's ordinary differential equation (9) in those rotated coordinates. We copy in the code for `isoGoal` and `isoCare` from [A8], since we are striving for high accuracy:

```
In[ ]:= memSqrt[z_ /; NumberQ[z]] := With[{s = Sqrt[z]},  
lastSqrt = If[Abs[lastSqrt + s] < Abs[lastSqrt - s], -s, s]]
```

```
isoGoal::novalidwp =  
"No warning-free value for the WorkingPrecision was found.";
```

```

isoGoal[{s_, t_}, g_] :=
Catch[
Do[Block[{lastSqrt = 1, res, q, r},
Quiet[Check[Quiet[
res = NDSolveValue[{
q'[r] ==
(((-bFr - I memSqrt[bEr bGr - bFr^2]) / bEr) /. {μ → q[r], ν → r}),
q[t] == s},
q, {r, 0, t},
AccuracyGoal → g, PrecisionGoal → Infinity,
WorkingPrecision → wp,
Method → If[g > 10, "StiffnessSwitching", Automatic]][0],
{NDSolveValue::precw}],
(* Always ignore this input-related warning. *)
res = Indeterminate]]; (* Discard the result
given any other warning. *)
If[NumberQ[res], Throw[res]]],
{wp, g + 5, 300, 5}];
Message[isoGoal::novalidwp]

```

```

isoCare::accfail = "Could not solve ODE to requested accuracy.";

```

```

isoCare[{s_, t_}, b_] :=
Catch[
Do[Block[{loAcc, mdAcc, hiAcc},
loAcc = isoGoal[{s, t}, g];
mdAcc = isoGoal[{s, t}, g + 5];
hiAcc = isoGoal[{s, t}, g + 10];
If[RealExponent[mdAcc - hiAcc] < RealExponent[loAcc - hiAcc] < -b ∨
loAcc == mdAcc == hiAcc == 0, (* result exactly zero is also okay *)
Throw[N[hiAcc, {Infinity, b}]]
]],
{g, b + 1, 300, 5}];
Message[isoCare::accfail]

```

To compute Poincaré coordinates from the resulting isothermal coordinates, we need to apply one of the refining polynomials  $C_{\text{deg}}$  from [A8]. Since we don't yet know which such polynomial will be needed, we read in the coefficients of all of the ones that were precomputed in [A8]. Those polynomials are stored in the data file "ApproximatingPolynomials.m", which is available, we assume, in the directory from which this package, "EquilateralPentagonMap.m", is being read.

```

degSeq = Union[Range[1, 25],
Range[25, 50, 5], Range[50, 100, 10], Range[100, 250, 25]];

```

```
ln[ ]:= dir =  
      If[$InputFileName == "", NotebookDirectory[], DirectoryName[$InputFileName]];
```

```
ln[ ]:= Get[FileNameJoin[{dir, "ApproximatingPolynomials.m"}]];
```

The input to  $C_{\text{deg}}$  is the complex output of  $\text{isoCare}$ , after we subtract  $2\pi/5$  from its real part to center the hypotenuse of the conformal image  $T_{\text{cnf}}$  at the origin. The output of  $C_{\text{deg}}$  lies in the triangle  $H_{\text{out}}$  in Figure 15. To convert that triangle into our output region  $T_{\text{out}}$ , we apply the hyperbolic isometry from above with  $\alpha = -\text{halfhyp}$  and  $\varphi = \pi/4$ , where

$$\text{halfhyp} = \sqrt{1 + \sqrt{5} + \sqrt{5 + 2\sqrt{5}}} - \sqrt{\sqrt{5} + \sqrt{5 + 2\sqrt{5}}}$$

$$\text{Out}[ ] = -\sqrt{\sqrt{5} + \sqrt{5 + 2\sqrt{5}}} + \sqrt{1 + \sqrt{5} + \sqrt{5 + 2\sqrt{5}}}$$

```
ln[ ]:= outputIsometry[z_] := ((1 + I) / Sqrt[2]) (z + halfhyp) / (1 + halfhyp z)
```

We have designed our algorithms to be accurate within  $T_{\text{in}}$ . As it happens, Gauss does just as well computing isothermal coordinates southeast of the main diagonal as northwest of it, and the polynomials  $C_{\text{deg}}$  also behave symmetrically across that diagonal. So we will be just as accurate when  $\xi > \eta$  as when  $\xi < \eta$ . But we do need to stay within the union of  $T_{\text{in}}$  and its reflection across its hypotenuse. The routine `goodPair` checks whether a point  $\{\xi, \eta\}$  lies within that union. (When checking the curved boundaries, we allow a small amount of slop,  $10^{-10}$ , to avoid ruling out floating-point pairs that actually do lie within that union.)

```
ln[ ]:= PoincareCoordinates::badPent =  
      "first arg must be widths of the two  
      narrowest sectors formed by the pentagon's five edges";
```

```
ln[ ]:= goodPair[{ξ_, η_}] := ξ ≥ 0 ∧ η ≥ 0 ∧  
      Cos[Min[ξ, η] / 2] - Cos[Max[ξ, η]] < 1 / 2 + 10^-10
```

```
ln[ ]:= PoincareCoordinates[{ξ_, η_} /; ! goodPair[{ξ, η}], acc_ : 17] :=  
      Message[PoincareCoordinates::badPent]
```

The second argument to `PoincareCoordinates` is the desired accuracy. We add 3 to that, to allow for rounding errors in the subsequent arithmetic and just to be on the safe side; and we compare the result to the computed max errors of our precomputed approximating polynomials, choosing the first of those whose accuracy is adequate. If none of those has sufficient accuracy, we issue a warning message.

```

In[ ]:= PoincareCoordinates::badAcc =
        "requested accuracy is too
        high for the precomputed approximating polynomials";

In[ ]:= degNeeded[acc_] := Catch[
        Do[If[-Lookup[poly[deg], maxLogErr] > acc + 3, Throw[deg]], {deg, degSeq}];
        Throw[NotAvailable]]

PoincareCoordinates[{ $\xi$  ? NumericQ,  $\eta$  ? NumericQ},
        acc_ /; (degNeeded[acc] == NotAvailable)] :=
        Message[PoincareCoordinates::badAcc]

```

The code for PoincareCoordinates in the non-error cases comes next. If the accuracy parameter is not specified, we default it to 17 decimal digits, which is roughly what you get in IEEE double precision.

```

PoincareCoordinates[{ $\xi$  ? NumericQ,  $\eta$  ? NumericQ}, acc_ : 17] :=
Module[{ $\mu$  =  $\eta + \xi$ ,  $\nu$  =  $\eta - \xi$ , deg = degNeeded[acc]},
  (* We evaluate the approximating polynomial  $C_{deg}$  using Horner's rule *)
  cPoly[z_] = Fold[z #1 + #2 &, 0, Table[c[deg - k], {k, 0, deg}]] /.
    Lookup[poly[deg], coeffVals];
  ReIm[outputIsometry[cPoly[isoCare[{ $\mu$ ,  $\nu$ }, acc] - 2  $\pi$  / 5]]]

```

Note that telling isoCare to solve the ODE in (9) with accuracy acc is adequate, since cPoly divides by about 6, which improves the accuracy of its output.

```

In[ ]:= End[];

In[ ]:= Protect[PoincareCoordinates];

In[ ]:= EndPackage[];

```

## A few tests

For a few easy tests of the function PoincareCoordinates, let's verify that the vertices of  $T_{\text{in}}$  are accurately mapped to the vertices of  $T_{\text{out}}$ . The  $\pi/4$  and  $\pi/5$  vertices get mapped quickly, even to high accuracy, because they are on the horizontal axis during the solution of the ODE in (9), and that axis is pointwise fixed:

```

In[ ]:= PoincareCoordinates[{0, 0}, 40]
Out[ ]:= {0.  $\times 10^{-41}$ , 0.  $\times 10^{-41}$ }

```

```
In[ ]:= PoincareCoordinates[{0, 0}, 100]
```

```
Out[ ]:= {0. × 10-101, 0. × 10-101}
```

```
In[ ]:= PoincareCoordinates[{72 Degree, 72 Degree}, 40]
```

```
Out[ ]:= {0.2814111230251358542050410267197685129376,  
0.2814111230251358542050410267197685129376}
```

```
In[ ]:= N[ $\frac{1}{2} \left( -5^{1/4} + \sqrt{2 + \sqrt{5}} \right)$ , 42]
```

```
Out[ ]:= 0.281411123025135854205041026719768512937635
```

```
In[ ]:= PoincareCoordinates[{72 Degree, 72 Degree}, 100]
```

```
Out[ ]:= {0.281411123025135854205041026719768512937635171031556570382474426296279078092\,  
6909563468363392197399593,  
0.281411123025135854205041026719768512937635171031556570382474426296279078092\,  
6909563468363392197399593}
```

```
In[ ]:= N[ $\frac{1}{2} \left( -5^{1/4} + \sqrt{2 + \sqrt{5}} \right)$ , 102]
```

```
Out[ ]:= 0.2814111230251358542050410267197685129376351710315565703824744262962790780926\,  
90956346836339219739959261
```

The  $\pi/2$  vertex provides a more interesting test, since it is a long way from the horizontal axis during the solution of the ODE in (9). Computing the Poincare coordinates of the transformed  $\pi/2$  vertex to 40 digits takes a couple of seconds, while computing it to 100 digits takes more than a minute:

```
In[ ]:= PoincareCoordinates[{0, 60 Degree}, 40]
```

```
Out[ ]:= {0. × 10-41, 0.2592635873236249780607534639561947829112}
```

```
In[ ]:= N[ $\sqrt{2 + \sqrt{5}} - \sqrt{1 + \sqrt{5}}$ , 42]
```

```
Out[ ]:= 0.259263587323624978060753463956194782911185
```

```
In[ ]:= PoincareCoordinates[{0, 60 Degree}, 100]
```

```
Out[ ]:= {0. × 10-101,  
0.259263587323624978060753463956194782911185116052605615686136920343872183357\,  
8458459297147027050364868}
```

```
In[ ]:= N[ $\sqrt{2 + \sqrt{5}} - \sqrt{1 + \sqrt{5}}$ , 102]
```

```
Out[ ]:= 0.2592635873236249780607534639561947829111851160526056156861369203438721833578\,  
45845929714702705036486847
```
